# Supplementary material for: Efficient algorithms for building representative matched pairs with enhanced generalizability
Source: arXiv:2205.04539 source file (2022-11-02)
Supplement: Supplementary file 1 [file online_supp.tex]

\clearpage
\pagenumbering{arabic}

\bigskip
  \bigskip
  \begin{center}
    {\LARGE\bf Online Supplemental Materials for ``Towards better reconciling randomized controlled trial and observational study findings: Efficient algorithms for building representative matched samples with enhanced external validity"}
 \end{center}

\captionsetup[table]{name=eTable}
\captionsetup[figure]{name=eFigure}
\setcounter{figure}{0}
\setcounter{table}{0}

\section*{Supplemental Material A: Statistical Matching, Network Flow, Recent Advancement}
Matching and subclassification are widely used in empirical research to embed noisy, non-randomized observational data into an approximate randomized controlled experiment, and facilitate analyzing data as such (\citealp{ho2007matching, rubin2007design,rubin2008objective,rosenbaum2002observational,rosenbaum2010design,rosenbaum2020modern,stuart2010matching,rassen2012one,imbens2015matching}). In a seminal paper, \citet{rosenbaum1989optimal} first bridged statistics literature on constructing matched samples and operations research and computer science literature on matching in graphs and networks. Prior to \citet{rosenbaum1989optimal}, statisticians and practitioners leveraged a ``greedy heuristic" in pair matching that starts with finding a matched pair with a minimum pre-specified distance, removes the pair from further consideration, and iterates the process until finding one control unit for each treated one in the study cohort. Some often-used distance metrics include the Mahalanobis distance in metric-based matching (\citealp{cochran1973controlling,rubin1980bias}), absolute difference in the estimated propensity score in propensity-score matching (\citealp{rosenbaum1983central}), or a combination of both (\citealp{rosenbaum1985constructing}).

\citet{rosenbaum1989optimal}'s key insight is to represent units to be matched, treated and control, as vertices in a bipartite graph and recast the statistical problem of constructing a matched control group as finding a minimum-cost network flow, a standard combinatorial optimization problem for which very efficient algorithms exist. Figure \ref{fig: bipartite schematic plot} illustrates this paradigm using a small example of three treated and five control units. Readers should imagine that the source node on the far left emits three units of flow, one unit arriving at the node $T_1$, one at $T_2$, and the other at $T_3$. Edges of the form $\textsf{e}(T_i, C_j)$ connecting $T_i$ and $C_j$, $i = 1, 2, 3$ and $j = 1, 2,..., 5$, each have capacity $1$ and are associated with a cost $\textsf{cost}\{\textsf{e}(T_i, C_j)\}$ equal to some covariate distance between $T_i$ and $C_j$. These three units of flow arriving at nodes $T_1$, $T_2$, and $T_3$ would choose to flow in such a way that minimizes the total cost; for instance, Figure \ref{fig: bipartite schematic plot} displays a minimum-cost flow (bold, black lines) consisting of $\{\textsf{e}(T_1, C_3), \textsf{e}(T_2, C_1), \textsf{e}(T_3, C_4)\}$. In this way, three matched pairs $\{(T_1, C_3), (T_2, C_1), (T_3, C_4)\}$ are constructed. The network structure displayed in Figure \ref{fig: bipartite schematic plot} can be readily modified to accommodate many useful design aspects, including exact matching, 1-to-$k$ matching, full matching (\citealp{hansen2004full,hansen2006optimal}), subset matching (\citealp{rosenbaum2007minimum}), among others, and is the cornerstone of some most influential statistical matching packages like \textsf{optmatch} (\citealp{hansen2007optmatch}) and \textsf{MatchIt} (\citealp{stuart2011matchit}) in the statistical computing software \textsf{R} (\citealp{team2013r}). Researchers have also proposed network-sparsification techniques to further facilitate statistical matching on large administrative datasets consisting of hundreds of thousands of observations (\citealp{pimentel2015large, yu2020matching}). 

More recently, \citet{zhang2021matching} introduced a minimum-cost network flow algorithm built around a ``tripartite graph," where treated units appear twice, on the far left and far right, with control units sandwiched between them. Efforts to balance high-dimensional covariates (e.g., via the stochastic balancing property of the propensity score or by directly minimizing the earthmover distance between marginal distributions) are represented on the right, while efforts to find close pairings (e.g., exact matching on potential effect modifiers or quantiles of \citet{hansen2008prognostic}'s prognostic score) are represented on the left. By separating two sometimes-conflicting objectives, pairing and balancing, the network built around a tripartite graph is shown to deliver matched samples that are homogeneous in a few key covariates while maintaining good balance in many other covariates (\citealp{zhang2021matching}).

\begin{figure}[ht]
\centering
\begin{tikzpicture}[thick, color = gray,
  every node/.style={draw,circle},
  fsnode/.style={fill=black, inner sep = 0pt, minimum size = 5pt},
  ssnode/.style={fill=gray, inner sep = 0pt, minimum size = 5pt},
  every fit/.style={ellipse,draw,inner sep=-2pt,text width=2cm},
  shorten >= 3pt,shorten <= 3pt
]

% the vertices of U

\begin{scope}[start chain=going below,node distance=8mm]
\foreach \i in {1,2,3}
  \node[fsnode,on chain] (t\i) [label=above: {\small$T_\i$} ] {};
\end{scope}

% the vertices of V
\begin{scope}[xshift=3.5cm,yshift=0cm,start chain=going below,node distance=8mm]
\foreach \i in {1,2,3,4,5}
  \node[ssnode,on chain] (c\i) [label=above: {\small$C_\i$}] {};
\end{scope}

\node [fill = black, inner sep = 0pt, minimum size = 5pt, label=left: \textsf{Source}] at (-2, -1) (source) {};

\node [fill = black, inner sep = 0pt, minimum size = 5pt, label=right: \textsf{Sink}] at (5.5, -2) (sink) {};

% the set U
%\node [blue,fit=(f1) (f5),label=above:$U$] {};
% the set V
%\node [green,fit=(s6) (s9),label=above:$V$] {};

% the edges
\draw (t1) -- (c1);
\draw (t1) -- (c2);
\draw [line width = 0.5mm, color = black] (t1) -- (c3);
\draw (t1) -- (c4);
\draw (t1) -- (c5);

\draw [line width = 0.5mm, color = black] (t2) -- (c1);
\draw (t2) -- (c2);
\draw (t2) -- (c3);
\draw (t2) -- (c4);
\draw (t2) -- (c5);

\draw (t3) -- (c1);
\draw (t3) -- (c2);
\draw (t3) -- (c3);
\draw [line width = 0.5mm, color = black] (t3) -- (c4);
\draw (t3) -- (c5);

\draw [line width = 0.5mm, color = black] (source) -- (t1);
\draw [line width = 0.5mm, color = black] (source) -- (t2);
\draw [line width = 0.5mm, color = black] (source) -- (t3);

\draw [line width = 0.5mm, color = black] (c1) -- (sink);
\draw (c2) -- (sink);
\draw [line width = 0.5mm, color = black] (c3) -- (sink);
\draw [line width = 0.5mm, color = black] (c4) -- (sink);
\draw (c5) -- (sink);
\end{tikzpicture}
\caption{Network-flow representation of a small matching problem. Five control units $C_1$, $C_2$, ..., $C_5$ are to be matched to three treated units $T_1$, $T_2$, and $T_3$. Each edge connecting $T_i$, $i = 1,2,3$, and $C_j$, $j = 1,2,3,4,5$, is associated with a flow capacity (equal to $1$ in pair matching) and a cost equal to a pre-specified covariate distance between unit $T_i$ and unit $C_j$.}
\label{fig: bipartite schematic plot}
\end{figure}

Representing statistical matching as a two-part network as depicted in Figure \ref{fig: bipartite schematic plot} is an attractive, general conceptual framework. Recent advancements in network-flow-based matching algorithms often involve adding an additional ``category" layer to the two-part network and using this additional layer to balance one or more nominal covariates in the treated and matched control groups (\citealp{rosenbaum1989optimal,yang2012optimal, pimentel2015large}). More recently, \citet{zhang2021matching} introduced a minimum-cost network flow algorithm built around a ``tripartite graph," where treated units appear twice, on the far left and far right, with control units sandwiched between them. Efforts to balance high-dimensional covariates (e.g., via the stochastic balancing property of the propensity score or by directly minimizing the earthmover's distance between marginal distributions) are represented on the right, while efforts to find close pairings (e.g., exact matching on potential effect modifiers or quantiles of \citet{hansen2008prognostic}'s prognostic score) are represented on the left. By separating two sometimes-conflicting objectives, pairing and balancing, the network built around a tripartite graph is shown to deliver matched samples that are homogeneous in a few key covariates while maintaining good balance in many other covariates (\citealp{zhang2021matching}).

\section*{Supplemental Material B: Additional Design and Computation Considerations}
Many additional design techniques can be used in conjunction with the proposed method by modifying aspects of the basic network structure in Figure \ref{fig: tripartite new scheme}. For instance, it is often helpful to match exactly on the potential effect modifiers in the design stage of an observational study, so that researchers could perform subgroup analysis by doing hypothesis testing in each stratum defined by the effect modifiers; see, e.g., \citet{lee2018discovering,lee2018powerful,lee2021discovering}. If such a design is desired, then researchers should set $\Delta_{\tau_t, \gamma_c}\{(\widetilde{\boldsymbol{x}}, \boldsymbol{x})\} = \infty$, or equivalently remove the edge connecting $\overline\tau_t$ and $\gamma_c$, for all $\tau_t$ and $\gamma_c$ disagreeing on the effect modifiers. \citet[Section 3.2]{rosenbaum1989optimal}'s fine balance strategy that forces equi-distribution of one nominal variable in the treated and matched control groups can also be readily accommodated by including an additional ``category" layer in the network; see also \citet{rosenbaum2007minimum, yang2012optimal, pimentel2015large,zhang2021matching}. In some practical situations, certain treated OBS units $\tau_t \in \mathcal{T}_{\textsf{sub}}$ are expected to be included in the matched samples. To achieve this, keep $\text{cost}\{(\tau_t, \overline\tau_t)\} = 0$ for $\tau_t \in \mathcal{T}_{\textsf{sub}}$ and set $\text{cost}\{(\tau_t, \overline\tau_t)\}$ to a large penalty for $\tau_t \in \mathcal{T}\backslash\mathcal{T}_{\textsf{sub}}$.

While the RCT is typically of a smaller, fixed sample size, modern observational databases could easily go beyond $1$ million observations. Consider a scenario with fixed RCT sample size $R$ and growing observational data sample sizes such that $T \rightarrow \infty$, $C \rightarrow \infty$, and $T/C \rightarrow \epsilon \in (0, 1)$. Recall the computation complexity of finding a minnimum cost flow is $O(|\mathcal{V}|\cdot|\mathcal{E}| + |\mathcal{V}|^2\log(|\mathcal{V}|))$. If the network can be made sparser so that $|\mathcal{E}| = O(|\mathcal{V}|\log(|\mathcal{V}|)) = O(C\log(C))$, then the complexity can be reduced from $O(C^3)$ to $O(C^2\log(C))$. One simplest way to sparsify the network is to leverage the propensity score caliper (\citealp{rosenbaum1985constructing,austin2011optimal}) and for each $\tau_t$, keep only edges of the form $e(\overline\tau_t, \gamma_c)$ for $C_1$ control units closest to $\tau_t$ in the estimated propensity score value. In this way, $|\mathcal{E}| = O(C_1 \cdot C)$, and the network is sparsified and computation complexity reduced provided $C_1 = O(\log C)$. Such a strategy is discussed in more detail in \citet{yu2020matching}.

\section*{Supplemental Material C: A Small Illustrative Example}
To showcase the utility of the proposed method, we consider a simple example where we generated a target RCT of size $R = 100$, and an observational study with $T = 500$ and $C = 1500$. The RCT collects $d_1 = 5$ covariates while the observational study collects an additional $5$ covariates. The RCT samples $\mathcal{K}$, OBS treated samples $\mathcal{T}$, and OBS control samples $\mathcal{C}$ have the same $\text{Normal}(0, 1)$ distribution for all but the first covariate $X_1$: $X_1 \sim \text{Normal}(0.25, 1)$ in the RCT samples, $X_1 \sim \text{Normal}(1, 1)$ in the OBS treated samples, and $X_1 \sim \text{Normal}(0, 1)$ in the OBS control samples. 

We considered three matched samples. In the first matched comparison, $500$ controls were matched to $500$ OBS treated units without heed of the target RCT covariate distributions. We matched this sample according to two criteria: (i) the earthmover's distance between the distributions of the estimated propensity score in the treated group and matched control group is minimized, and (ii) subject to (i), the total robust Mahalanobis distances between treated and control units are minimized (\citealp{zhang2021matching}). We refer to this match $\textsf{M1}$. In the second matched comparison, we leveraged the proposed new network structure in Figure \ref{fig: tripartite new scheme} with $k = 1$ and $\lambda = 1$ and formed $100$ treated-to-control matched pairs. In this second match, we specified $\delta_{\kappa_r, \tau_t} (\widetilde{\boldsymbol{x}})$ as the absolute difference in the estimated generalizability score between $\kappa_r$ and $\tau_t$ in $5$ RCT covariates, and let $\Delta_{\tau_t, \gamma_c}\{(\widetilde{\boldsymbol{x}}, \boldsymbol{x})\}$ be the robust Mahalanobis distance within a $0.05$ estimated propensity score caliper between $\tau_t$ and $\gamma_c$ in all $10$ covariates. We refer to this match $\textsf{M2}$. The third match $\textsf{M3}$ used the same network structure and distance specifications as $\textsf{M2}$, but with $k = 2$ so that $200$ treated-to-control pairs were formed.

Figure \ref{fig: illustrative example} displays the covariate distributions of three matched samples. Before matching, the treated and control groups are vastly different in $X_1$ but otherwise similar. Match $\textsf{M1}$ does a good job balancing $X_1$ via balancing the estimated propensity score; see the third boxplot in the left panel of Figure \ref{fig: illustrative example}. However, despite within-matched-samples close resemblance, the treated group $\mathcal{T}$ and matched controls produced by $\textsf{M1}$ differ systematically from the target template in the distribution of $X_1$. The $100$ matched pairs returned by $\textsf{M2}$ not only have good within-matched-sample-homogeneity, but also are much more similar to the target template in covariates' distributions. The same pattern holds for the $200$ matched pairs returned by $\textsf{M3}$.

\begin{figure}[ht]
   \centering
     \subfloat{\includegraphics[width = 0.49\columnwidth]{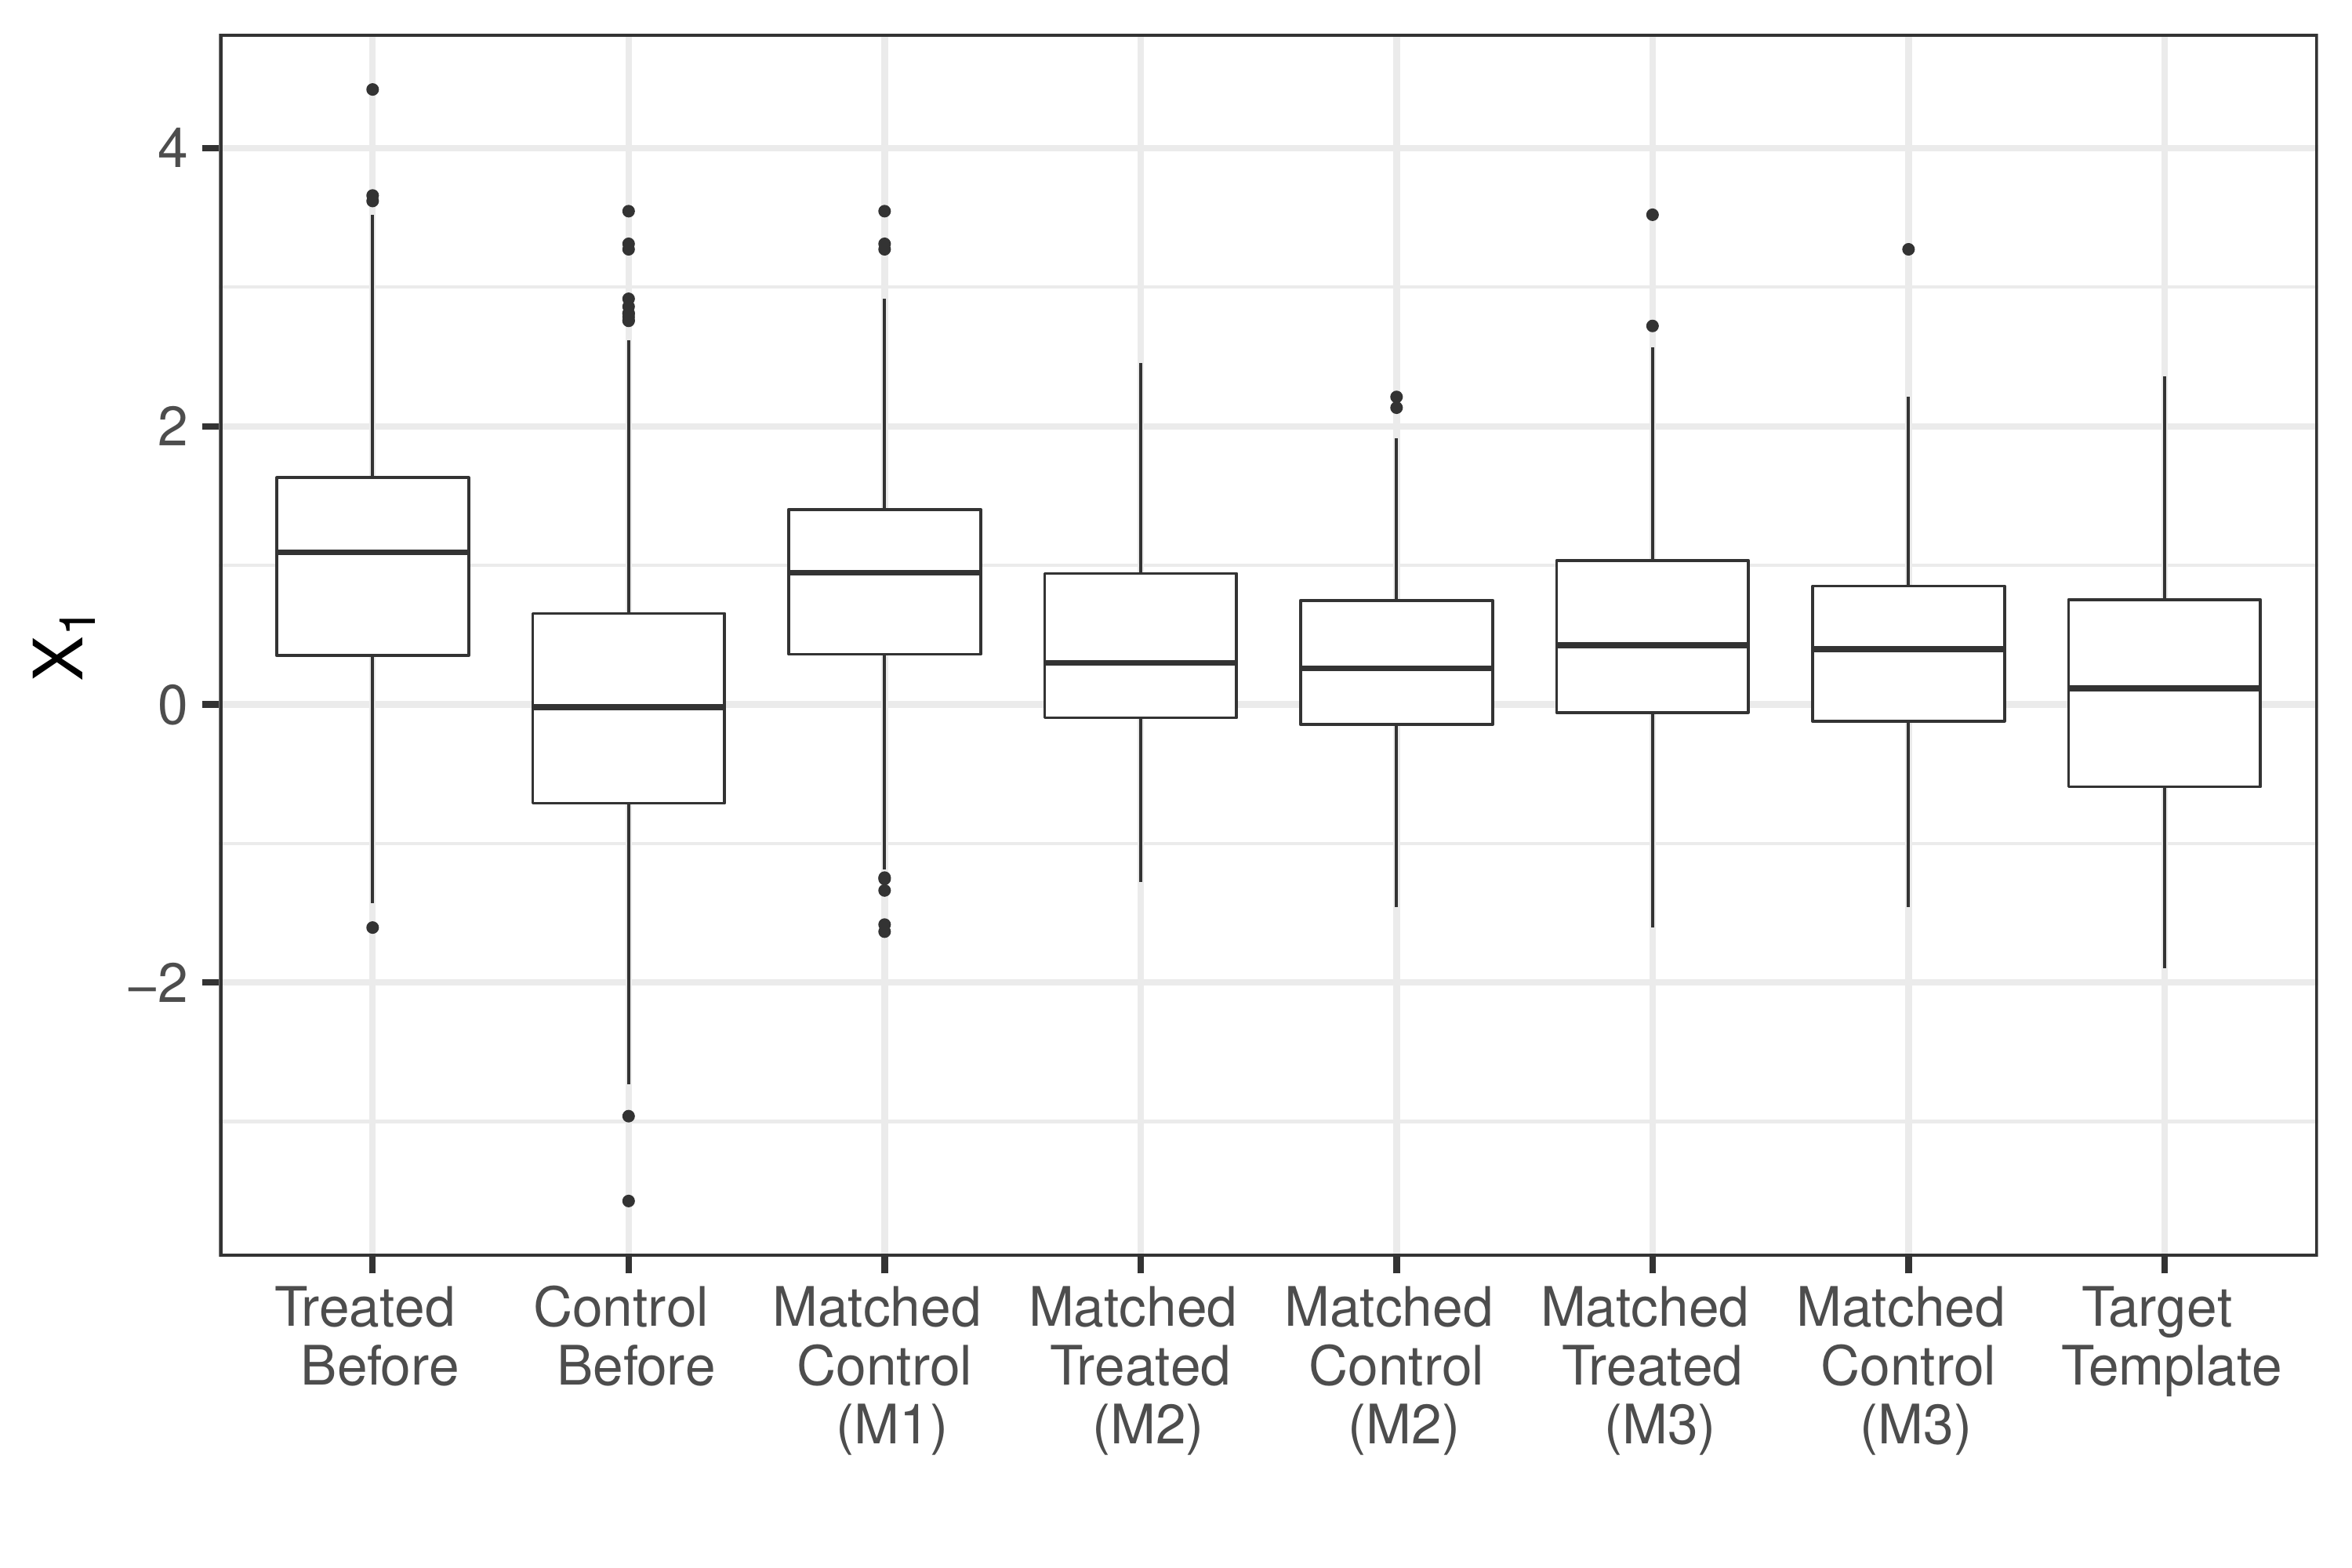}}
     \subfloat{\includegraphics[width = 0.49\columnwidth]{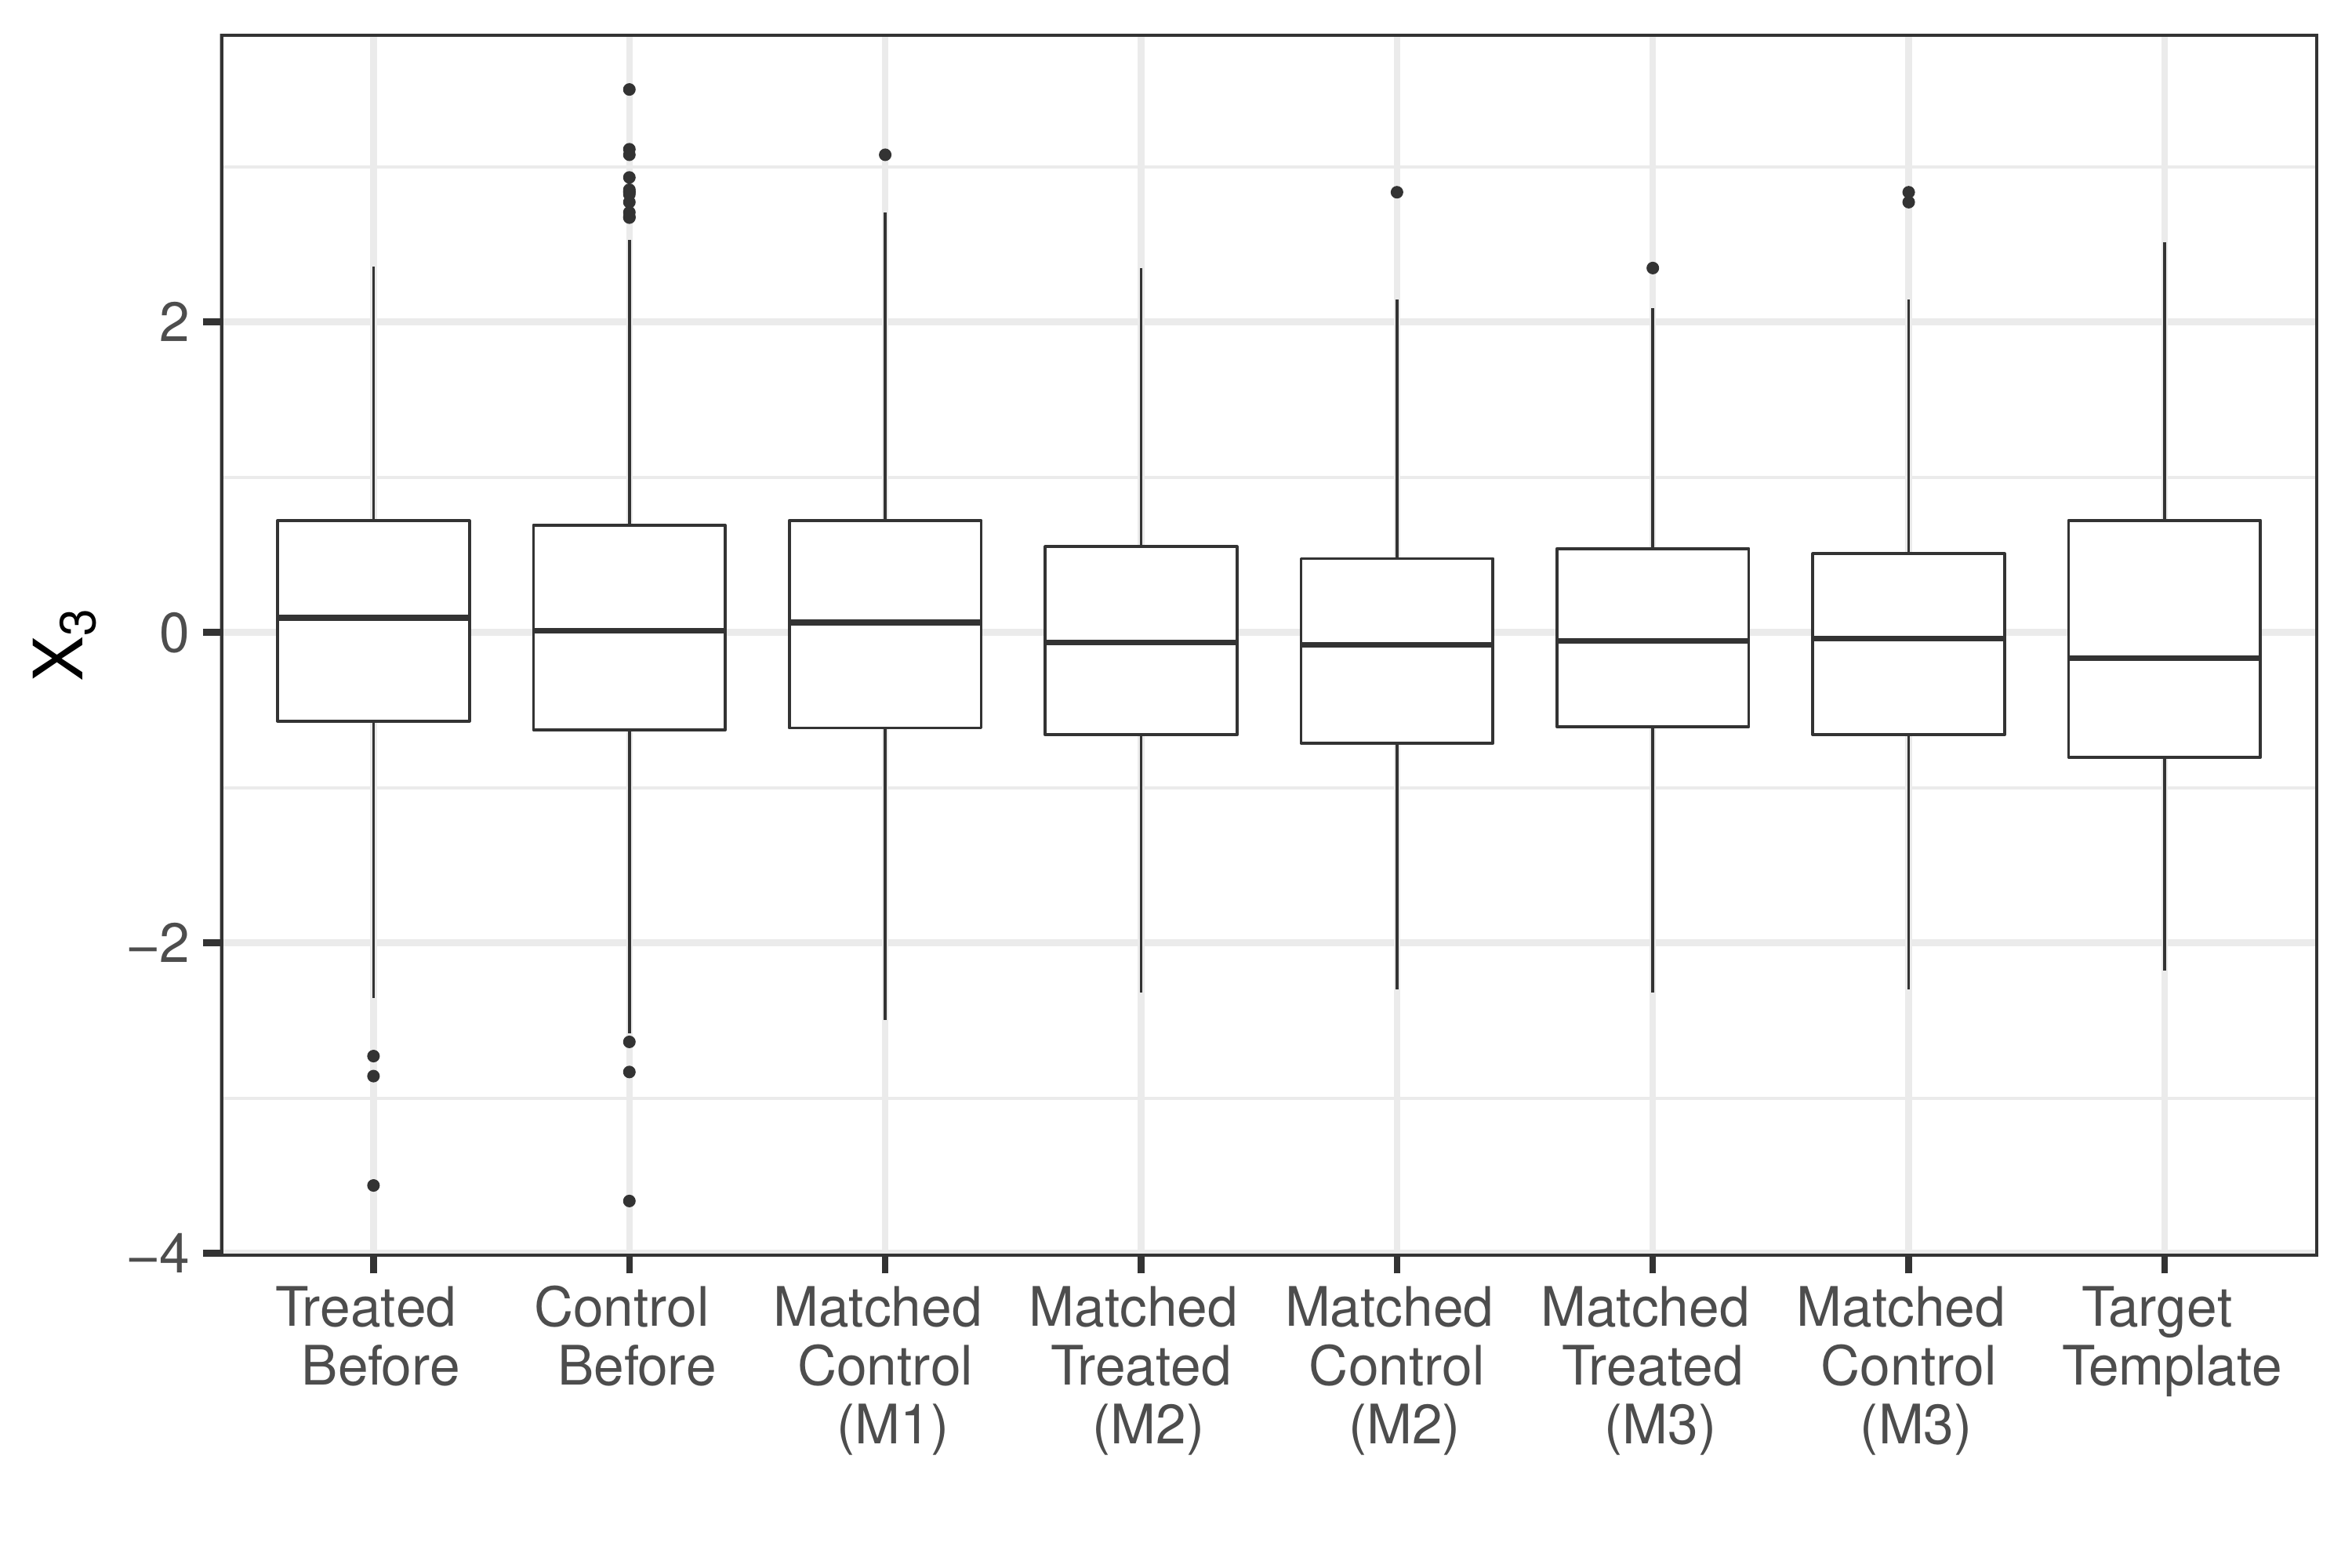}}
     \caption{Comparing the distributions of covariates $X_1$ (left panel) and $X_3$ (right panel) in three matched comparisons.}
\label{fig: illustrative example}
\end{figure}

\section*{Supplemental Material D: Simulation Studies}
\subsection*{D.1: Goal, Structure, Measurement of Success}
Our primary goal in this section is to examine how the study design delivered by different matching algorithms affects the performance of downstream statistical inference. In particular, we are interested in the case where the treatment effect is heterogeneous and the distributions of effect modifiers vary in the observational database and the target template. We generated a template $\mathcal{K}$ with $|\mathcal{K}| = 300$ and $\mathbf{X} \sim \text{Multivariate Normal}\left(\mathbf\mu, \mathbf \Sigma\right)$, with $\mathbf \mu = (0.25, 0, 0, 0, 0)^{\text{T}}$ and $\mathbf\Sigma = \mathbf I_{5\times 5}$. We consider an observational database with $|\mathcal{T}| = 1000$ treated and $|\mathcal{C}| = 3000$ control units. The data-generating process for units in the observational database and statistical matching procedures to be investigated are specified via the following factorial design:
\begin{description}
\item \textbf{Factor 1:} Dimension of covariates in the observational database, $d$: $10$, $30$, and $50$.
\item \textbf{Factor 2:} Overlap between template, treated ($Z = 1$), and control ($Z = 0$) units, $\beta$: 
$\mathbf{X} \sim \text{Multivariate Normal}\left(\mathbf\mu, \mathbf \Sigma\right)$, with $\mathbf \mu = (\theta Z, 0, 0, 0, 0)^{\text{T}}$ and $\mathbf\Sigma = \mathbf I_{d\times d}$. We consider $\theta = 0.25$, $0.50$, and $1$.

\item \textbf{Factor 3:} Matching algorithms to be investigated, $\mathcal{M}$: 
\begin{enumerate}
    \item $\mathcal{M}_{\textsf{opt}}$: matching according to two criteria (\citealp{zhang2021matching}): (i) minimizing the earthmover's distance between the distributions of the estimated propensity score in the treated and matched control groups, and (ii) subject to (i), minimizing the within-matched-pair robust Mahalanobis distances. Algorithm $\mathcal{M}_{\textsf{opt}}$ produces $1000$ matched pairs, and pays no attention to the target template.
    
    \item $\mathcal{M}_{\textsf{template},~k = 1}$: matching according to the proposed network structure (Figure \ref{fig: tripartite new scheme}) with $k = 1$. Algorithm $\mathcal{M}_{\textsf{template},~k = 1}$ produces $300$ matched pairs.
   
    \item $\mathcal{M}_{\textsf{template},~k = 2}$: similar to $\mathcal{M}_{\textsf{template},~k = 1}$ but with $k = 2$. Algorithm $\mathcal{M}_{\textsf{template},~k = 2}$ produces $600$ matched pairs.
\end{enumerate}

\item \textbf{Factor 4:} Tuning parameter in $\mathcal{M}_{\textsf{template},~k}$, $\lambda$: $100$, $1$, $0.01$.
\end{description}

Factor $1$ and $2$ define the data-generating process for units in the observational database. Factor $3$ and $4$ define a total of $1 + 2 \times 3 = 7$ matching algorithms under consideration. As discussed in Section \ref{subsec: tradeoff}, the tuning parameter $\lambda$ controls the trade-off between internal and external validity of effect estimates obtained from matched samples. 

For each unit, we further generate two potential outcomes according to the following data-generating process:
\begin{equation}
    \label{eq: simu outcome}
    Y(0) \sim N(0, 1),\qquad Y(1) = Y(0) + \beta(X_1),
\end{equation}
and the observed outcome satisfies $Y = Z\cdot Y(1) + (1-Z)\cdot Y(0)$. The last factor specifies the treatment effect:
\begin{description}
\item \textbf{Factor 5:} Treatment effect, $\beta(X_1)$: a constant treatment effect $\beta(X_1) = 2$, a mildly heterogeneous treatment effect $\beta(X_1) = 2 - 0.2X_1$, and a strongly heterogeneous treatment effect $\beta(X_1) = 2 - X_1$. 
\end{description}
When the treatment effect is heterogeneous and the effect modifier $X_1$ has a different distribution in the RCT group and the OBS treated group, then the average treated effect on the treated (ATT) estimate obtained from the matched observational study cannot be automatically generalized to the RCT cohort (\citealp{stuart2011use}). 

There are multiple ways to analyze matched pair data. Examples include parametric t-test, randomization inference (\citealp{rosenbaum2002observational,rosenbaum2010design}), and regression adjustment (\citealp{rubin1979using, ho2007matching}). In this simulation study, we report a simple difference-in-means estimator for matched data produced by each of the $7$ algorithms, and compare these $7$ effect estimates to the treatment effect averaged over the target template, i.e., $\textsf{SATE}_{\text{target}}$. We report the average bias and mean squared error of each of the $7$ effect estimates against $\textsf{SATE}_{\text{target}}$.

\subsection*{D.2: Simulation Results}
Table \ref{tbl: simulation results b = 1} summarizes the percentage of bias with respect to $\textsf{SATE}_{\text{target}}$ of each difference-in-means estimator $\widehat{\theta}_{\mathcal{M}}$ obtained from matched samples constructed from algorithm $\mathcal{M}$. 

%Simulation results on the mean squared error are similar and can be found in the Supplementary Material \textcolor{red}{XX}.

We have observed a few trends consistent with both theory and intuition. First, when the treatment is constant, there is no generalizability issue and the bias is minuscule under all data-generating processes and statistical matching algorithms under consideration. Second, when the treatment effect is heterogeneous and the effect modifier $X_1$ has a different distribution in the template and the treated units, effect estimate obtained from $1000$ matched pairs constructed using algorithm $\mathcal{M}_{\textsf{opt}}$ is clearly biased from $\textsf{SATE}_{\text{target}}$, and the percentage of bias increases (i) as the distributions of $X_1$ become increasingly dissimilar in the target template and in the OBS treated units (i.e., as $b$ increases), and (ii) as effect modification becomes more dramatic (i.e., from constant to mild to strong). In the most adversarial setting considered in this simulation study, i.e., when $b = 1$ and $\beta(X_1) = 2 - X_1$, the percentage bias of $\widehat{\theta}_{\mathcal{M}_{\textsf{opt}}}$ can be as large as $45\%$. We need to stress that although $\widehat{\theta}_{\mathcal{M}_{\textsf{opt}}}$ may not be generalized to the target template, it is a perfectly internally-valid estimator for the treatment effect averaged over covariates' distributions of OBS treated units.

Our proposed template matching algorithms outperform $\mathcal{M}_{\textsf{opt}}$ in bias reduction against $\textsf{SATE}_{\text{target}}$ in all $6$ different implementations under all data-generating processes considered in this simulation study, although the gain in bias reduction differs from implementation to implementation. In particular, we observe that the gain is most pronounced when (i) $k$ is small so that a smaller treated group bearing more resemblance to the target template is constructed, and (ii) $\lambda$ is large so that the matching algorithm gives more priority to the left part compared to the right part of the network depicted in Figure \ref{fig: tripartite new scheme}, i.e., resemblance to the target template in covariates' distributions is emphasized over resemblance between matched treated and matched control groups. Both parameters, $k$ and $\lambda$, effectively allow a trade-off between the internal validity of a matched observational study and its generalizability to a target population. Matching is part of the design of an observational study and should be carried out without looking at the outcome data. Good practice includes keeping time-stamped analysis logs for review and posting a detailed pre-analysis protocol; see, e.g., \cite{franklin2020nonrandomized, franklin2021emulating}. Provided that no outcome data are viewed, researchers can feel free to perform multiple statistical matching and select the one achieving the best trade-off between internal and external validity in an real world problem.

\begin{table}[ht]
\centering
\caption{Percentage of bias with respect to $\textsf{SATE}_{\text{target}}$ of $7$ difference-in-means estimator constructed from matched samples obtained from each of the $7$ matching algorithms. Each cell is averaged over $1000$ simulations.}
\label{tbl: simulation results b = 1}
\resizebox{0.9\textwidth}{!}{
\begin{tabular}{cccccccccccc}\hline \\ [-0.8em]\multirow{3}{*}{\begin{tabular}{c}Heterogeneity \\ Level\end{tabular}}
&\multirow{3}{*}{\begin{tabular}{c}$b$\end{tabular}}&& \multirow{3}{*}{\begin{tabular}{c}$\mathcal{M}_{\textsf{opt}}$\end{tabular}} 
&& \multicolumn{6}{c}{$\mathcal{M}_{\textsf{template}}$} \\ \\ [-0.8em] \cline{6-11} \\ [-0.8em]
&&&& & \multirow{2}{*}{\begin{tabular}{c}$k = 1$ \\ $\lambda = 0.01$ \end{tabular}}  
& \multirow{2}{*}{\begin{tabular}{c}$k = 1$ \\ $\lambda = 1$ \end{tabular}} 
& \multirow{2}{*}{\begin{tabular}{c}$k = 1$ \\ $\lambda = 100$ \end{tabular}} 
& \multirow{2}{*}{\begin{tabular}{c}$k = 2$ \\ $\lambda = 0.01$ \end{tabular}}  
& \multirow{2}{*}{\begin{tabular}{c}$k = 2$ \\ $\lambda = 1$ \end{tabular}} 
& \multirow{2}{*}{\begin{tabular}{c}$k = 2$ \\ $\lambda = 100$ \end{tabular}} \\ \\ \\ [-0.8em]
    \multicolumn{11}{c}{$d = 10$} \\ \\ [-0.8em]
    
    % Constant
    \multirow{3}{*}{Constant} &0.25
    && 0.001 && 0.000 & 0.001 & 0.001 & 0.001 & 0.000 & 0.001 \\ 
    &0.50 && 0.000 && 0.001 & 0.001 & 0.001 & 0.001 & 0.000 & 0.000 \\ 
    & 1.00 && 0.000 && 0.002 & 0.000 & 0.001 & 0.000 & 0.000 & 0.000 \\ \\ [-0.8em]

       \multirow{3}{*}{Mild} &0.25
   && 0.007 && 0.003 & 0.000 & 0.002 & 0.004 & 0.001 & 0.002 \\ 
  &0.50 && 0.033 && 0.009 & 0.008 & 0.018 & 0.011 & 0.012 & 0.020 \\ 
  &1.00 && 0.084 && 0.019 & 0.020 & 0.044 & 0.034 & 0.034 & 0.050 \\ \\ [-0.8em]

 %Strong
  \multirow{3}{*}{Strong} &0.25
  && 0.042 && 0.007 & 0.003 & 0.001 & 0.011 & 0.006 & 0.010 \\ 
 &0.50 && 0.177 && 0.041 & 0.035 & 0.086 & 0.055 & 0.050 & 0.103 \\ 
 &1.00 && 0.451 && 0.102 & 0.098 & 0.223 & 0.188 & 0.186 & 0.262 \\ \\ [-0.8em]
     \multicolumn{11}{c}{$d = 30$} \\  \\ [-0.8em]
         % Constant
          \multirow{3}{*}{Constant} &0.25
    && 0.000 && 0.003 & 0.000 & 0.001 & 0.000 & 0.000 & 0.000 \\ 
    &0.50 && 0.001 && 0.001 & 0.001 & 0.002 & 0.001 & 0.002 & 0.002 \\ 
    &1.00 && 0.001 && 0.001 & 0.000 & 0.001 & 0.000 & 0.001 & 0.002 \\ \\ [-0.8em]
    % Mild
     \multirow{3}{*}{Mild} &0.25
    && 0.008 && 0.003 & 0.003 & 0.004 & 0.003 & 0.003 & 0.005 \\ 
    &0.50 && 0.031 && 0.008 & 0.009 & 0.015 & 0.009 & 0.013 & 0.019 \\ 
    &1.00 && 0.084 && 0.019 & 0.025 & 0.037 & 0.036 & 0.039 & 0.048 \\ \\ [-0.8em]
  % Strong
   \multirow{3}{*}{Strong} &0.25
  && 0.042 && 0.007 & 0.007 & 0.012 & 0.010 & 0.012 & 0.020 \\ 
 &0.50 && 0.178 && 0.040 & 0.058 & 0.095 & 0.053 & 0.080 & 0.114 \\ 
 &1.00 && 0.452 && 0.105 & 0.137 & 0.207 & 0.189 & 0.214 & 0.259 \\ \\ [-0.8em]
  \multicolumn{11}{c}{$d = 50$} \\  \\ [-0.8em]
  % Constant
   \multirow{3}{*}{Constant} &0.25
  && 0.001 && 0.000 & 0.001 & 0.001 & 0.001 & 0.001 & 0.001 \\ 
 &0.50 && 0.001 && 0.002 & 0.001 & 0.001 & 0.002 & 0.000 & 0.000 \\ 
 &1.00 && 0.000 && 0.000 & 0.001 & 0.000 & 0.001 & 0.001 & 0.001 \\ \\ [-0.8em]
  % Mild
   \multirow{3}{*}{Mild} &0.25
  && 0.006 && 0.001 & 0.001 & 0.001 & 0.002 & 0.001 & 0.003 \\ 
 &0.50 && 0.034 && 0.008 & 0.011 & 0.017 & 0.010 & 0.016 & 0.021 \\ 
 &1.00 && 0.084 && 0.019 & 0.028 & 0.038 & 0.035 & 0.042 & 0.049 \\ \\ [-0.8em]
  % Strong
   \multirow{3}{*}{Strong} &0.25
  && 0.040 && 0.007 & 0.006 & 0.013 & 0.009 & 0.014 & 0.021 \\ 
 &0.50 && 0.178 && 0.038 & 0.065 & 0.095 & 0.053 & 0.088 & 0.113 \\ 
 &1.00 && 0.451 && 0.102 & 0.150 & 0.205 & 0.188 & 0.224 & 0.260 \\ \\ [-0.8em] \hline
\end{tabular}}
\end{table}

\clearpage
\section*{Supplemental Material E: More Details on the WHI Case Study}
\subsection*{E.1: Plot of the Estimated Propensity Score}

\begin{figure}[ht]
    \centering
    \includegraphics[width=\textwidth]{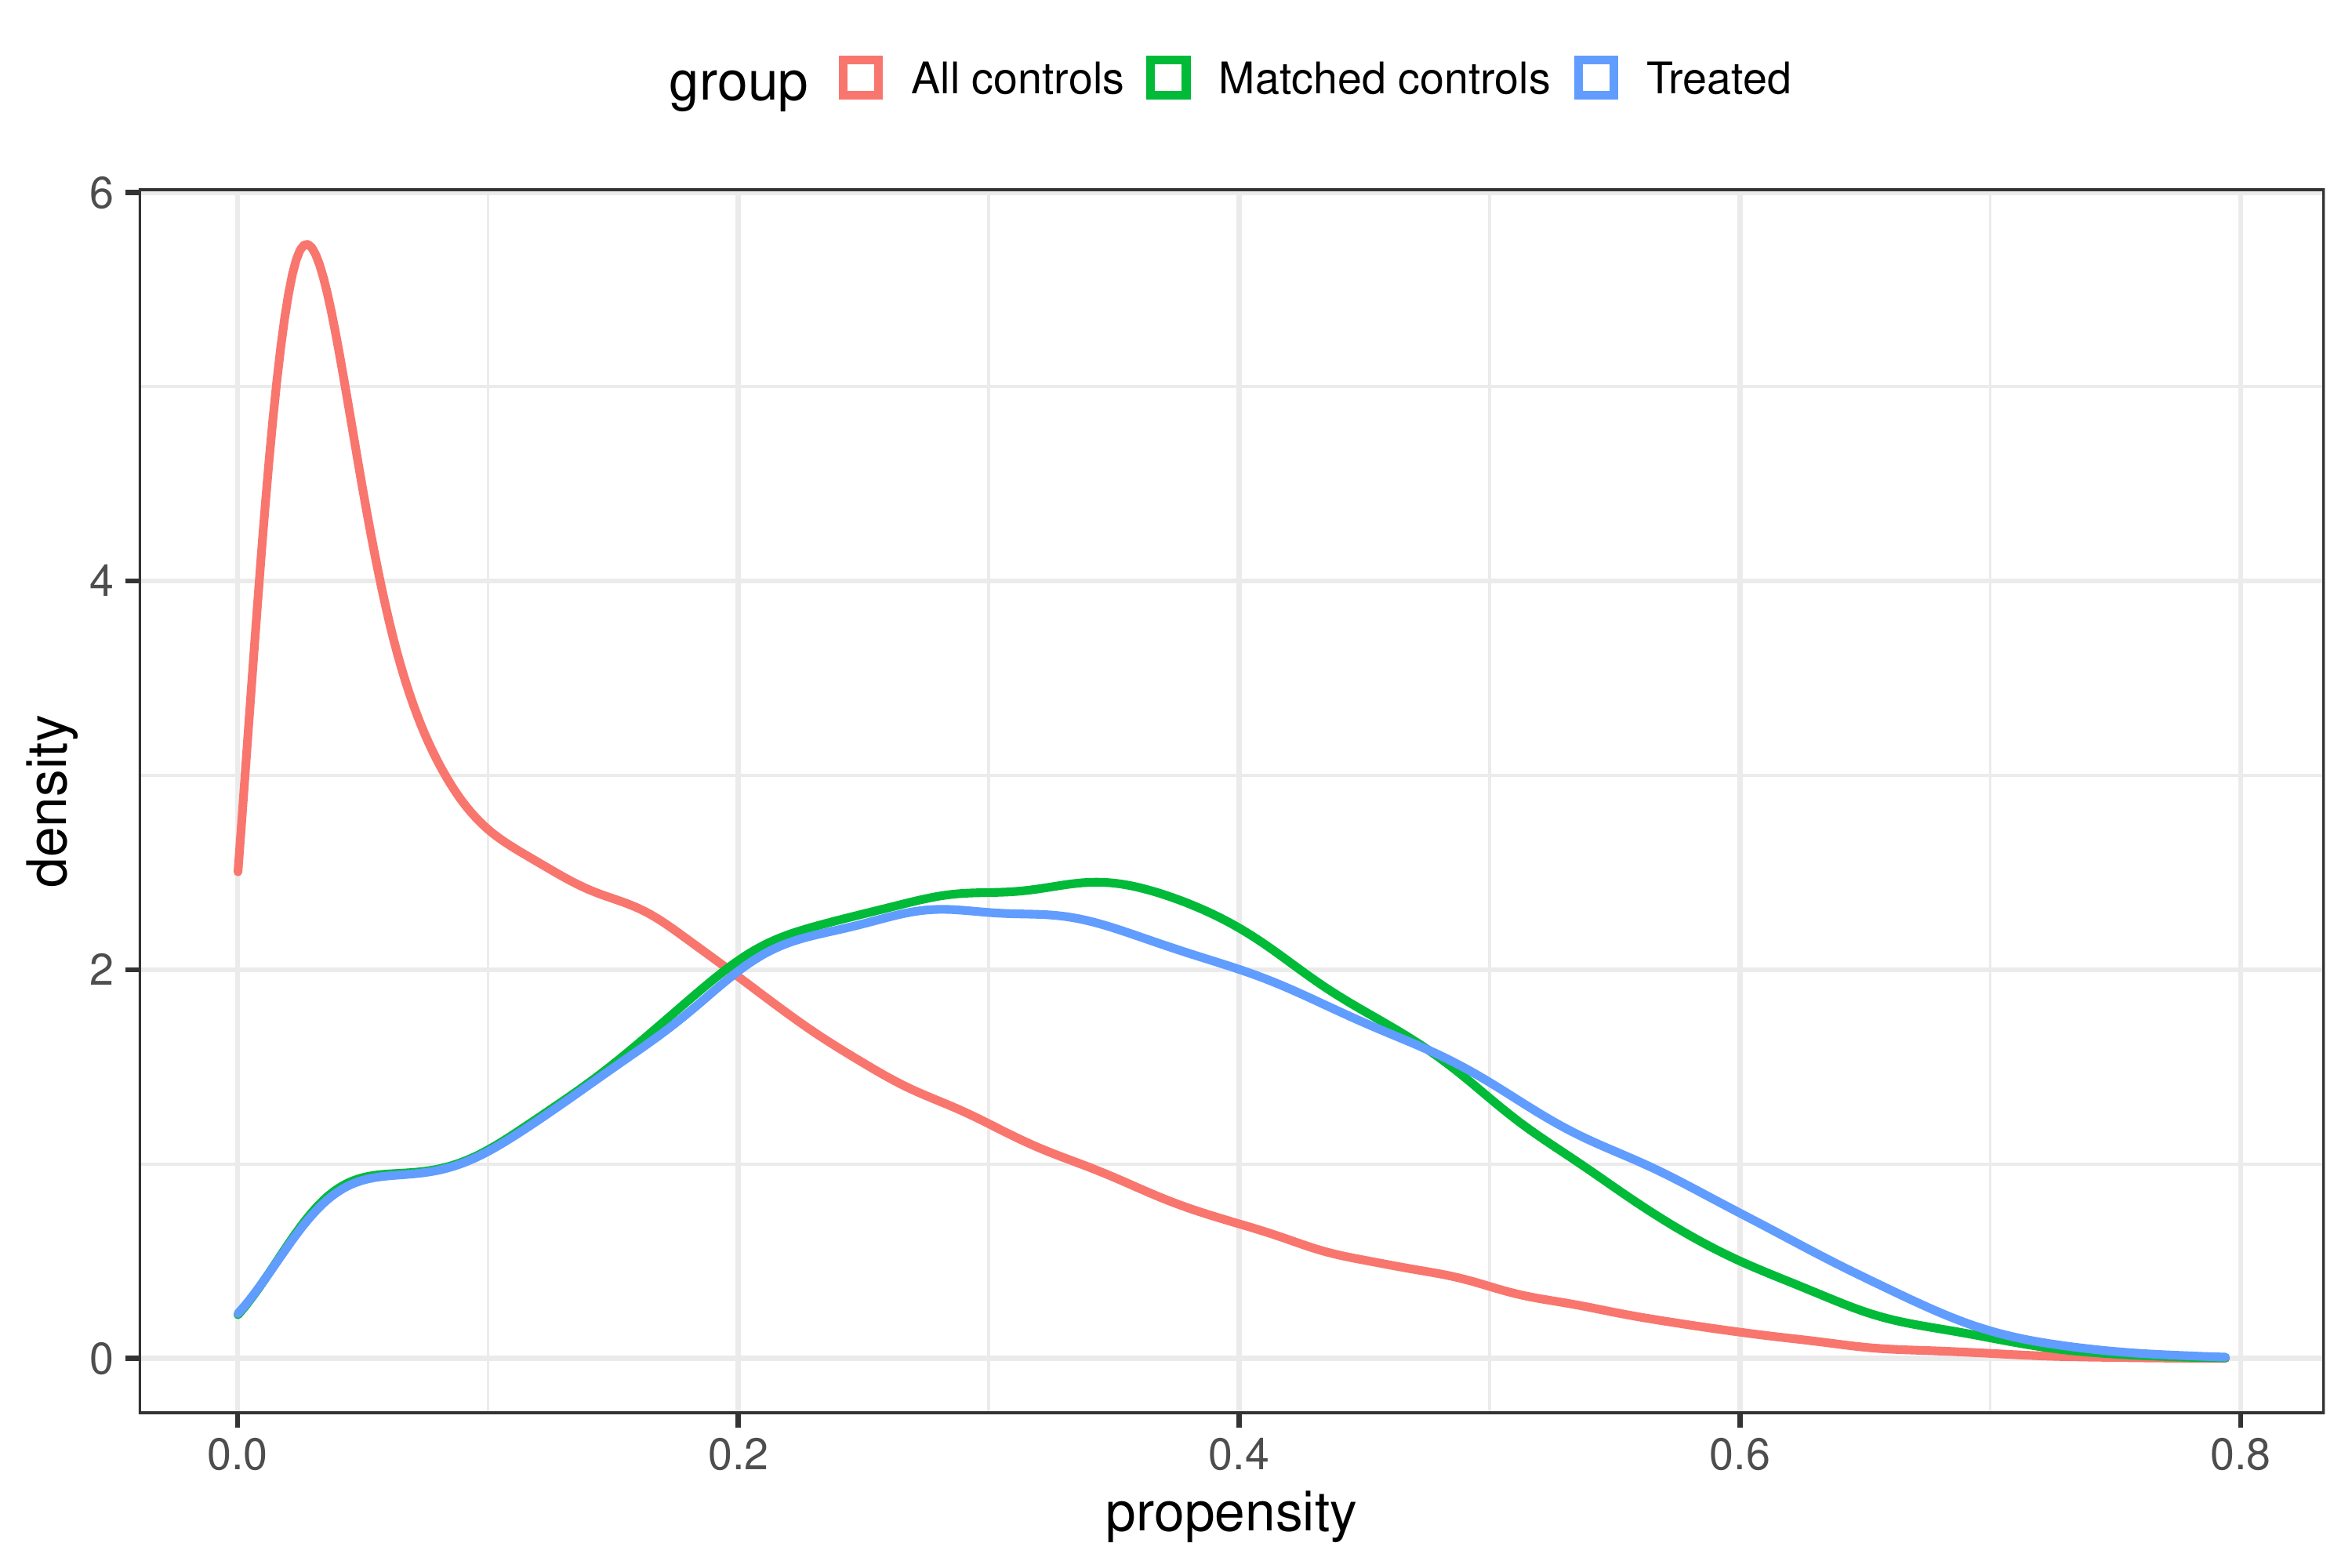}
    \caption{Distributions of the estimated propensity score in the entire treated OBS group (blue), the entire control OBS group (red), and the matched control group (green).}
\end{figure}

\subsection*{E.2: Balance table of $\textsf{M0}$}

\begin{table}[H]
\centering
\caption{\small Balance table before matching and of $18,340$ matched pairs in the match $\textsf{M0}$}
\label{tbl: matched samples I}
\resizebox{0.78\textwidth}{!}{
\begin{tabular}{lccccccccc}
  \hline
  &\multirow{4}{*}{\begin{tabular}{c}\textbf{OBS} \\ \textbf{Treated} \\ \textbf{(n = 18340)}\end{tabular}} 
    &\multirow{4}{*}{\begin{tabular}{c}\textbf{OBS} \\ \textbf{Control} \\ \textbf{(n = 75303)}\end{tabular}}
        &\multirow{4}{*}{\begin{tabular}{c}\textbf{SMD} \\ \textbf{Before}\end{tabular}}
     &\multirow{4}{*}{\begin{tabular}{c}\textbf{Matched} \\ \textbf{Control} \\\textbf{(n=18340)}\end{tabular}}
   &\multirow{4}{*}{\begin{tabular}{c}\textbf{SMD} \\ \textbf{M0}\end{tabular}}
   \\ \\ \\ \\ \\ [-0.6em]
   
   \multicolumn{6}{c}{\large\textbf{HRT Prior Usage}}\\  \\ [-0.6em]
   \textbf{Age at initiation} \\
   \hspace{0.2cm}NA & 0 &0.89 & &0.85\\
   \hspace{0.2cm}Age & 53.87 &52.04 & & 51.75\\
   \textbf{Previous E+P use, yrs} & 7.02 & 0.47 & &0.55 &  \\ \\ [-0.6em]
   
   \multicolumn{6}{c}{\large\textbf{Covariates Collected in RCT and OBS}}\\  \\ [-0.6em]
\textbf{Age at screening} & 60.84 & 64.30 & -0.35 & 61.10 & -0.03 \\ 
\textbf{Race/Ethnicity}\\
 \hspace{0.2cm}White & 0.89 & 0.82 & 0.14 & 0.89 & -0.00 \\ 
   \hspace{0.2cm}Black/Hispanic & 0.06 & 0.14 & -0.18 & 0.06 & 0.00 \\  
   \textbf{Education}\\
 \hspace{0.2cm}College or above & 0.55 & 0.40 & 0.21 & 0.55 & 0.00 \\ 
  \hspace{0.2cm} Some college & 0.32 & 0.37 & -0.08 & 0.32 & 0.00 \\ 
  \hspace{0.2cm} High school diploma/GED & 0.11 & 0.17 & -0.13 & 0.11 & -0.00 \\ 
  \textbf{Blood pressure}\\
  \hspace{0.2cm}Systolic & 123.27 & 127.86 & -0.19 & 123.54 & -0.01 \\ 
  \hspace{0.2cm}Diastolic & 74.03 & 74.91 & -0.07 & 74.23 & -0.02 \\
  \textbf{BMI} & 25.85 & 27.61 & -0.22 & 25.99 & -0.02 \\
 \textbf{Smoking}\\
 \hspace{0.2cm}Current smoker & 0.05 & 0.06 & -0.04 & 0.05 & 0.00 \\ 
  \hspace{0.2cm}Never smoked & 0.47 & 0.51 & -0.05 & 0.48 & -0.00 \\  
  \hspace{0.2cm}Past smoker & 0.46 & 0.41 & 0.07 & 0.46 & 0.00 \\ 
  \textbf{No. of PA episodes}\\
  \hspace{0.2cm}Total & 5.80 & 5.29 & 0.09 & 5.74 & 0.01 \\ 
  \hspace{0.2cm}Medium to strenuous & 3.58 & 2.94 & 0.13 & 3.50 & 0.02 \\ \\
   \multicolumn{6}{c}{\large\textbf{Additional OBS Covariates}}\\  \\ [-0.6em]
  \textbf{Region}\\
  \hspace{0.2cm}Midwest & 0.22 & 0.22 & 0.00 & 0.23 & -0.01 \\ 
  \hspace{0.2cm}Northeast & 0.18 & 0.24 & -0.09 & 0.19 & -0.02 \\
  \hspace{0.2cm}South & 0.25 & 0.26 & -0.02 & 0.25 & 0.00 \\ 
     \textbf{Partner's education}\\
  \hspace{0.2cm}College or above & 0.43 & 0.30 & 0.20 & 0.42 & 0.02 \\ 
  \hspace{0.2cm}Some college & 0.16 & 0.17 & -0.01 & 0.17 & -0.01 \\  
   \hspace{0.2cm}High school diploma/GED & 0.07 & 0.09 & -0.05 & 0.07 & -0.00 \\ 
   \textbf{Income}\\
   \hspace{0.2cm}Below 35K & 0.23 & 0.40 & -0.26 & 0.24 & -0.01 \\ 
   \hspace{0.2cm} 35K - 75K & 0.42 & 0.36 & 0.09 & 0.44 & -0.02 \\  
   \hspace{0.2cm}Above 75K & 0.29 & 0.16 & 0.22 & 0.27 & 0.04 \\ 
   \textbf{Marital status}\\
   \hspace{0.2cm}Married & 0.69 & 0.60 & 0.13 & 0.69 & 0.01 \\
   \hspace{0.2cm}Divorced/Widowed & 0.26 & 0.35 & -0.13 & 0.27 & -0.01 \\ 
 \textbf{Employment status}\\
  \hspace{0.2cm}Yes & 0.45 & 0.32 & 0.19 & 0.45 & -0.00 \\ 
  \hspace{0.2cm}No & 0.53 & 0.65 & -0.17 & 0.53 & 0.00 \\  
\textbf{Reproductive history}\\  
  \hspace{0.2cm}No ovary removed & 0.92 & 0.64 & 0.51 & 0.92 & 0.00 \\ 
\hspace{0.2cm}Oral contraceptive use ever & 0.53 & 0.37 & 0.24 & 0.53 & 0.00 \\ 
  \hspace{0.2cm}OC duration in years & 5.59 & 5.16 & 0.09 & 5.41 & 0.04 \\
  \textbf{Preexisting Conditions}\\
  \hspace{0.2cm}Stroke & 0.01 & 0.02 & -0.08 & 0.00 & 0.01 \\ 
  \hspace{0.2cm}MI  & 0.01 & 0.03 & -0.07 & 0.01 & 0.00 \\ 
  \hspace{0.2cm}CHF & 0.00 & 0.01 & -0.06 & 0.00 & 0.00 \\
  \hspace{0.2cm}Liver diseases & 0.02 & 0.02 & -0.02 & 0.02 & -0.01 \\
  \hspace{0.2cm}Hypertension & 0.25 & 0.35 & -0.16 & 0.25 & -0.00 \\ 
  \hspace{0.2cm}Fracture & 0.10 & 0.14 & -0.09 & 0.11 & -0.01 \\ 
  \hspace{0.2cm}CABG/PTCA & 0.01 & 0.02 & -0.05 & 0.01 & 0.00 \\
  \hspace{0.2cm}BRCA & 0.01 & 0.07 & -0.22 & 0.01 & 0.00 \\ 
   \hline
\end{tabular}}
\end{table}
