# Supplementary material for: Efficient algorithms for building representative matched pairs with enhanced generalizability
Source: arXiv:2205.04539 source file (2022-11-02)
Supplement: Supplementary file 2 [file appendix.tex]

\subsection{Statistical Matching, Network Flow, Recent Advancement}
%In an observational study of a treatment's effect on an outcome, units receiving and not receiving the treatment often differ systematically in their observed covariates, thus invalidating a naive comparison. 
\textcolor{red}{Move this section to the Appendix.}

Matching and subclassification are widely used in empirical research to embed noisy, non-randomized observational data into an approximate randomized controlled experiment, and facilitate analyzing data as such (\citealp{ho2007matching, rubin2007design,rubin2008objective,rosenbaum2002observational,rosenbaum2010design,rosenbaum2020modern,stuart2010matching,rassen2012one,imbens2015matching}). In a seminal paper, \citet{rosenbaum1989optimal} first bridged statistics literature on constructing matched samples and operations research and computer science literature on matching in graphs and networks. Prior to \citet{rosenbaum1989optimal}, statisticians and practitioners leveraged a ``greedy heuristic" in pair matching that starts with finding a matched pair with a minimum pre-specified distance, removes the pair from further consideration, and iterates the process until finding one control unit for each treated one in the study cohort. Some often-used distance metrics include the Mahalanobis distance in metric-based matching (\citealp{cochran1973controlling,rubin1980bias}), absolute difference in the estimated propensity score in propensity-score matching (\citealp{rosenbaum1983central}), or a combination of both (\citealp{rosenbaum1985constructing}).

\citet{rosenbaum1989optimal}'s key insight is to represent units to be matched, treated and control, as vertices in a bipartite graph and recast the statistical problem of constructing a matched control group as finding a minimum-cost network flow, a standard combinatorial optimization problem for which very efficient algorithms exist. Figure \ref{fig: bipartite schematic plot} illustrates this paradigm using a small example of three treated and five control units. Readers should imagine that the source node on the far left emits three units of flow, one unit arriving at the node $T_1$, one at $T_2$, and the other at $T_3$. Edges of the form $\textsf{e}(T_i, C_j)$ connecting $T_i$ and $C_j$, $i = 1, 2, 3$ and $j = 1, 2,..., 5$, each have capacity $1$ and are associated with a cost $\textsf{cost}\{\textsf{e}(T_i, C_j)\}$ equal to some covariate distance between $T_i$ and $C_j$. These three units of flow arriving at nodes $T_1$, $T_2$, and $T_3$ would choose to flow in such a way that minimizes the total cost; for instance, Figure \ref{fig: bipartite schematic plot} displays a minimum-cost flow (bold, black lines) consisting of $\{\textsf{e}(T_1, C_3), \textsf{e}(T_2, C_1), \textsf{e}(T_3, C_4)\}$. In this way, three matched pairs $\{(T_1, C_3), (T_2, C_1), (T_3, C_4)\}$ are constructed. The network structure displayed in Figure \ref{fig: bipartite schematic plot} can be readily modified to accommodate many useful design aspects, including exact matching, 1-to-$k$ matching, full matching (\citealp{hansen2004full,hansen2006optimal}), subset matching (\citealp{rosenbaum2007minimum}), among others, and is the cornerstone of some most influential statistical matching packages like \textsf{optmatch} (\citealp{hansen2007optmatch}) and \textsf{MatchIt} (\citealp{stuart2011matchit}) in the statistical computing software \textsf{R} (\citealp{team2013r}). Researchers have also proposed network-sparsification techniques to further facilitate statistical matching on large administrative datasets consisting of hundreds of thousands of observations (\citealp{pimentel2015large, yu2020matching}). 

More recently, \citet{zhang2021matching} introduced a minimum-cost network flow algorithm built around a ``tripartite graph," where treated units appear twice, on the far left and far right, with control units sandwiched between them. Efforts to balance high-dimensional covariates (e.g., via the stochastic balancing property of the propensity score or by directly minimizing the earthmover distance between marginal distributions) are represented on the right, while efforts to find close pairings (e.g., exact matching on potential effect modifiers or quantiles of \citet{hansen2008prognostic}'s prognostic score) are represented on the left. By separating two sometimes-conflicting objectives, pairing and balancing, the network built around a tripartite graph is shown to deliver matched samples that are homogeneous in a few key covariates while maintaining good balance in many other covariates (\citealp{zhang2021matching}).

\begin{figure}[ht]
\centering
\begin{tikzpicture}[thick, color = gray,
  every node/.style={draw,circle},
  fsnode/.style={fill=black, inner sep = 0pt, minimum size = 5pt},
  ssnode/.style={fill=gray, inner sep = 0pt, minimum size = 5pt},
  every fit/.style={ellipse,draw,inner sep=-2pt,text width=2cm},
  shorten >= 3pt,shorten <= 3pt
]

% the vertices of U

\begin{scope}[start chain=going below,node distance=8mm]
\foreach \i in {1,2,3}
  \node[fsnode,on chain] (t\i) [label=above: {\small$T_\i$} ] {};
\end{scope}

% the vertices of V
\begin{scope}[xshift=3.5cm,yshift=0cm,start chain=going below,node distance=8mm]
\foreach \i in {1,2,3,4,5}
  \node[ssnode,on chain] (c\i) [label=above: {\small$C_\i$}] {};
\end{scope}

\node [fill = black, inner sep = 0pt, minimum size = 5pt, label=left: \textsf{Source}] at (-2, -1) (source) {};

\node [fill = black, inner sep = 0pt, minimum size = 5pt, label=right: \textsf{Sink}] at (5.5, -2) (sink) {};

% the set U
%\node [blue,fit=(f1) (f5),label=above:$U$] {};
% the set V
%\node [green,fit=(s6) (s9),label=above:$V$] {};

% the edges
\draw (t1) -- (c1);
\draw (t1) -- (c2);
\draw [line width = 0.5mm, color = black] (t1) -- (c3);
\draw (t1) -- (c4);
\draw (t1) -- (c5);

\draw [line width = 0.5mm, color = black] (t2) -- (c1);
\draw (t2) -- (c2);
\draw (t2) -- (c3);
\draw (t2) -- (c4);
\draw (t2) -- (c5);

\draw (t3) -- (c1);
\draw (t3) -- (c2);
\draw (t3) -- (c3);
\draw [line width = 0.5mm, color = black] (t3) -- (c4);
\draw (t3) -- (c5);

\draw [line width = 0.5mm, color = black] (source) -- (t1);
\draw [line width = 0.5mm, color = black] (source) -- (t2);
\draw [line width = 0.5mm, color = black] (source) -- (t3);

\draw [line width = 0.5mm, color = black] (c1) -- (sink);
\draw (c2) -- (sink);
\draw [line width = 0.5mm, color = black] (c3) -- (sink);
\draw [line width = 0.5mm, color = black] (c4) -- (sink);
\draw (c5) -- (sink);
\end{tikzpicture}
\caption{Network-flow representation of a small matching problem. Five control units $C_1$, $C_2$, ..., $C_5$ are to be matched to three treated units $T_1$, $T_2$, and $T_3$. Each edge connecting $T_i$, $i = 1,2,3$, and $C_j$, $j = 1,2,3,4,5$, is associated with a flow capacity (equal to $1$ in pair matching) and a cost equal to a pre-specified covariate distance between unit $T_i$ and unit $C_j$.}
\label{fig: bipartite schematic plot}
\end{figure}

%Representing statistical matching as a two-part network as depicted in Figure \ref{fig: bipartite schematic plot} is an attractive, general conceptual framework. Recent advancements in network-flow-based matching algorithms often involve adding an additional ``category" layer to the two-part network and using this additional layer to balance one or more nominal covariates in the treated and matched control groups (\citealp{rosenbaum1989optimal,yang2012optimal, pimentel2015large}). More recently, \citet{zhang2021matching} introduced a minimum-cost network flow algorithm built around a ``tripartite graph," where treated units appear twice, on the far left and far right, with control units sandwiched between them. Efforts to balance high-dimensional covariates (e.g., via the stochastic balancing property of the propensity score or by directly minimizing the earthmover's distance between marginal distributions) are represented on the right, while efforts to find close pairings (e.g., exact matching on potential effect modifiers or quantiles of \citet{hansen2008prognostic}'s prognostic score) are represented on the left. By separating two sometimes-conflicting objectives, pairing and balancing, the network built around a tripartite graph is shown to deliver matched samples that are homogeneous in a few key covariates while maintaining good balance in many other covariates (\citealp{zhang2021matching}).

\subsection{A Naive Method, An Existing Method, and A New Approach}
One naive approach to create homogeneous matched pairs resembling a target template would first select a subset of treated units from the observational data via matching on covariates collected by both RCT and observational study. In the second step, control units in the observational data are then matched to the treated units selected by the first step. This strategy suffers from a major drawback. Take the RCT DUPLICATE initiative as an example. Although the benchmark SAVOR-TIMI 53 trial reported only around $20$ baseline covariates, \citet{franklin2021emulating} matched on more than $120$ to guard against unmeasured confounding in their emulation with observational data. In the first step, there are many ways to design a smaller treated group similar to the RCT population in $20$ RCT covariates; however, it is difficult to determine which treated group designed from the first step should be utilized to form the eventual match in the second step. A selected treated group similar to the RCT population in $20$ RCT covariates could have poor overlap with the control units in the observational database in the other more than $100$ covariates; see Figure \ref{fig: illustrate naive method} for a toy example that illustrates this phenomenon. Ideally, we prefer well-matched treated and control groups using observational data to first ensure internal validity of the matched cohort study; similarity to some target population should be taken as a perk. The naive approach precludes a principled trade-off between matched cohort study's internal validity and its generalizability to a target population.

\begin{figure}[ht]
    \centering
   \begin{tikzpicture}

% Template
\node at (0.25, 1.25) {$X_1$};
\node at (1, 1.25) {$X_2$};
\draw[blue, very thick] (0,0) rectangle (0.5,0.5);
\draw[blue, very thick] (1,0.25) circle (0.25);
\node[text width=2cm, align = center] at (0.6, -4) {\small\textsf{Template}};

% Obs treated
\node at (4.25, 1.25) {$X_1$};
\node at (5, 1.25) {$X_2$};
\node at (5.75, 1.25) {$X_3$};

\node at (3.25,0.25) {$\textsf{T1}$};
\node at (3.25,-0.5) {$\textsf{T2}$};
\draw[blue, very thick] (4,0) rectangle (4.5,0.5);
\draw[blue, very thick] (5,0.25) circle (0.25);
\draw[blue, very thick] (5.75,0.25) circle (0.25);

\draw[blue, very thick] (4,-0.75) rectangle (4.5,-0.25);
\draw[blue, very thick] (5,-0.5) circle (0.25);
\draw[blue, very thick] (5.5,-0.75) -- (5.75,-0.25) -- (6,-0.75) -- cycle;

\node[text width=2cm, align = center] at (5, -4) {\small\textsf{OBS \\ Treated}};

% OBS control
\node at (9, 1.25) {$X_1$};
\node at (9.75, 1.25) {$X_2$};
\node at (10.5, 1.25) {$X_3$};

\node at (8,0.25) {$\textsf{C1}$};
\node at (8,-0.5) {$\textsf{C2}$};
\node at (8,-1.25) {$\textsf{C3}$};
\node at (8,-2) {$\textsf{C4}$};

\draw[blue, very thick] (9,0.25) circle (0.25);
\draw[blue, very thick] (9.75,0.25) circle (0.25);
\draw[blue, very thick] (10.5,0.25) circle (0.25);

\draw[blue, very thick] (8.75,-0.75) rectangle (9.25,-0.25);
\draw[blue, very thick] (9.75,-0.5) circle (0.25);
\draw[blue, very thick] (10.5,-0.5) circle (0.25);

\draw[blue, very thick] (8.75,-1.5) rectangle (9.25,-1);
\draw[blue, very thick] (9.75,-1.25) circle (0.25);
\draw[blue, very thick] (10.25,-1.5) rectangle (10.75, -1);

\draw[blue, very thick] (8.75,-2.25) rectangle (9.25,-1.75);
\draw[blue, very thick] (9.5,-2.25) rectangle (10, -1.75);
\draw[blue, very thick] (10.25,-2.25) rectangle (10.75, -1.75);

\node[text width=2cm, align = center] at (9.75, -4) {\small\textsf{OBS \\ Control}};

\end{tikzpicture}
\caption{A toy example illustrating the limitation of a naive two-step approach. Suppose our goal is to create one treated-to-control pair. In the first step, treated units are matched to the template to obtain a candidate treated group. In this toy example, both $\textsf{T1}$ and $\textsf{T2}$ are good match to the template judging from two RCT covariates $X_1$ and $X_2$. However, in view of the reservoir of control units, $\textsf{T1}$ is a better pick as no control unit has an $X_3$ value similar to that of $\textsf{T2}$.}
\label{fig: illustrate naive method}
\end{figure}

Recently, \citet{bennett2020building} developed a mixed-integer-programming-based (MIP-based) approach that builds representative matched samples. MIP-based matching algorithms (\citealp{li2001balanced,zubizarreta2012using,bennett2020building}) are more flexible compared to network-flow-based ones as requirements for different versions of covariate balance could be readily represented by constraints in a mathematical program. Although recent advancements in computing power have made it more practical to solve large-scale MIP problems with many complex constraints, the general MIP problems are still theoretically intractable or NP-hard. From a very practical perspective, MIP-based methods require installing a powerful commercial optimization routine (e.g., Gurobi or IBM CPLEX), and this is itself an obstacle to some empirical researchers. This being said, if one finds no difficulty installing a powerful solver and that the matching task can be readily solved using MIP-based methods, then this is great and one should do that.

Compared to MIP-based methods, network-flow-based methods only require solving a polynomial solvable problem that is tractable both in theory and practice, and have proven successful in empirical comparative effectiveness research for decades (\citealp{rosenbaum2002observational,rosenbaum2010design, stuart2010matching, austin2011introduction,rassen2012one}). The primary goal of this article is to outline an efficient, easy-to-use, network-flow-based algorithm that designs matched pairs from observational data with close resemblance to a target population. We demonstrate the usefulness of the proposed method by revisiting the Women's Health Initiative (WHI) study, and explore how the method facilitates different designs of the WHI observational study data and yields some useful, new insight into the well-aged inconsistency between WHI trial and observational study findings.

\subsection{Additional Design and Computation Considerations}
\label{subsec: additional design considerations}
Many additional design techniques can be used in conjunction with the proposed method by modifying aspects of the basic network structure in Figure \ref{fig: tripartite new scheme}. For instance, it is often helpful to match exactly on the potential effect modifiers in the design stage of an observational study, so that researchers could perform subgroup analysis by doing hypothesis testing in each stratum defined by the effect modifiers; see, e.g., \citet{lee2018discovering,lee2018powerful,lee2021discovering}. If such a design is desired, then researchers should set $\Delta_{\tau_t, \gamma_c}\{(\widetilde{\boldsymbol{x}}, \boldsymbol{x})\} = \infty$, or equivalently remove the edge connecting $\overline\tau_t$ and $\gamma_c$, for all $\tau_t$ and $\gamma_c$ disagreeing on the effect modifiers. \citet[Section 3.2]{rosenbaum1989optimal}'s fine balance strategy that forces equi-distribution of one nominal variable in the treated and matched control groups can also be readily accommodated by including an additional ``category" layer in the network; see also \citet{rosenbaum2007minimum, yang2012optimal, pimentel2015large,zhang2021matching}. In some practical situations, certain treated OBS units $\tau_t \in \mathcal{T}_{\textsf{sub}}$ are expected to be included in the matched samples. To achieve this, keep $\text{cost}\{(\tau_t, \overline\tau_t)\} = 0$ for $\tau_t \in \mathcal{T}_{\textsf{sub}}$ and set $\text{cost}\{(\tau_t, \overline\tau_t)\}$ to a large penalty for $\tau_t \in \mathcal{T}\backslash\mathcal{T}_{\textsf{sub}}$.

While the RCT is typically of a smaller, fixed sample size, modern observational databases could easily go beyond $1$ million observations. Consider a scenario with fixed RCT sample size $R$ and growing observational data sample sizes such that $T \rightarrow \infty$, $C \rightarrow \infty$, and $T/C \rightarrow \epsilon \in (0, 1)$. Recall the computation complexity of finding a minnimum cost flow is $O(|\mathcal{V}|\cdot|\mathcal{E}| + |\mathcal{V}|^2\log(|\mathcal{V}|))$. If the network can be made sparser so that $|\mathcal{E}| = O(|\mathcal{V}|\log(|\mathcal{V}|)) = O(C\log(C))$, then the complexity can be reduced from $O(C^3)$ to $O(C^2\log(C))$. One simplest way to sparsify the network is to leverage the propensity score caliper (\citealp{rosenbaum1985constructing,austin2011optimal}) and for each $\tau_t$, keep only edges of the form $e(\overline\tau_t, \gamma_c)$ for $C_1$ control units closest to $\tau_t$ in the estimated propensity score value. In this way, $|\mathcal{E}| = O(C_1 \cdot C)$, and the network is sparsified and computation complexity reduced provided $C_1 = O(\log C)$. Such a strategy is discussed in more detail in \citet{yu2020matching}.

\subsection{A Small Illustrative Example}
\label{subsec: a small example}
\textcolor{red}{Perhaps do a subsection on software and implementation.}
To showcase the utility of the proposed method, we consider a simple example where we generated a target RCT of size $R = 100$, and an observational study with $T = 500$ and $C = 1500$. The RCT collects $d_1 = 5$ covariates while the observational study collects an additional $5$ covariates. The RCT samples $\mathcal{K}$, OBS treated samples $\mathcal{T}$, and OBS control samples $\mathcal{C}$ have the same $\text{Normal}(0, 1)$ distribution for all but the first covariate $X_1$: $X_1 \sim \text{Normal}(0.25, 1)$ in the RCT samples, $X_1 \sim \text{Normal}(1, 1)$ in the OBS treated samples, and $X_1 \sim \text{Normal}(0, 1)$ in the OBS control samples. 

We considered three matched samples. In the first matched comparison, $500$ controls were matched to $500$ OBS treated units without heed of the target RCT covariate distributions. We matched this sample according to two criteria: (i) the earthmover's distance between the distributions of the estimated propensity score in the treated group and matched control group is minimized, and (ii) subject to (i), the total robust Mahalanobis distances between treated and control units are minimized (\citealp{zhang2021matching}). We refer to this match $\textsf{M1}$. In the second matched comparison, we leveraged the proposed new network structure in Figure \ref{fig: tripartite new scheme} with $k = 1$ and $\lambda = 1$ and formed $100$ treated-to-control matched pairs. In this second match, we specified $\delta_{\kappa_r, \tau_t} (\widetilde{\boldsymbol{x}})$ as the absolute difference in the estimated generalizability score between $\kappa_r$ and $\tau_t$ in $5$ RCT covariates, and let $\Delta_{\tau_t, \gamma_c}\{(\widetilde{\boldsymbol{x}}, \boldsymbol{x})\}$ be the robust Mahalanobis distance within a $0.05$ estimated propensity score caliper between $\tau_t$ and $\gamma_c$ in all $10$ covariates. We refer to this match $\textsf{M2}$. The third match $\textsf{M3}$ used the same network structure and distance specifications as $\textsf{M2}$, but with $k = 2$ so that $200$ treated-to-control pairs were formed.

Figure \ref{fig: illustrative example} displays the covariate distributions of three matched samples. Before matching, the treated and control groups are vastly different in $X_1$ but otherwise similar. Match $\textsf{M1}$ does a good job balancing $X_1$ via balancing the estimated propensity score; see the third boxplot in the left panel of Figure \ref{fig: illustrative example}. However, despite within-matched-samples close resemblance, the treated group $\mathcal{T}$ and matched controls produced by $\textsf{M1}$ differ systematically from the target template in the distribution of $X_1$. The $100$ matched pairs returned by $\textsf{M2}$ not only have good within-matched-sample-homogeneity, but also are much more similar to the target template in covariates' distributions. The same pattern holds for the $200$ matched pairs returned by $\textsf{M3}$.

\begin{figure}[ht]
   \centering
     \subfloat{\includegraphics[width = 0.49\columnwidth]{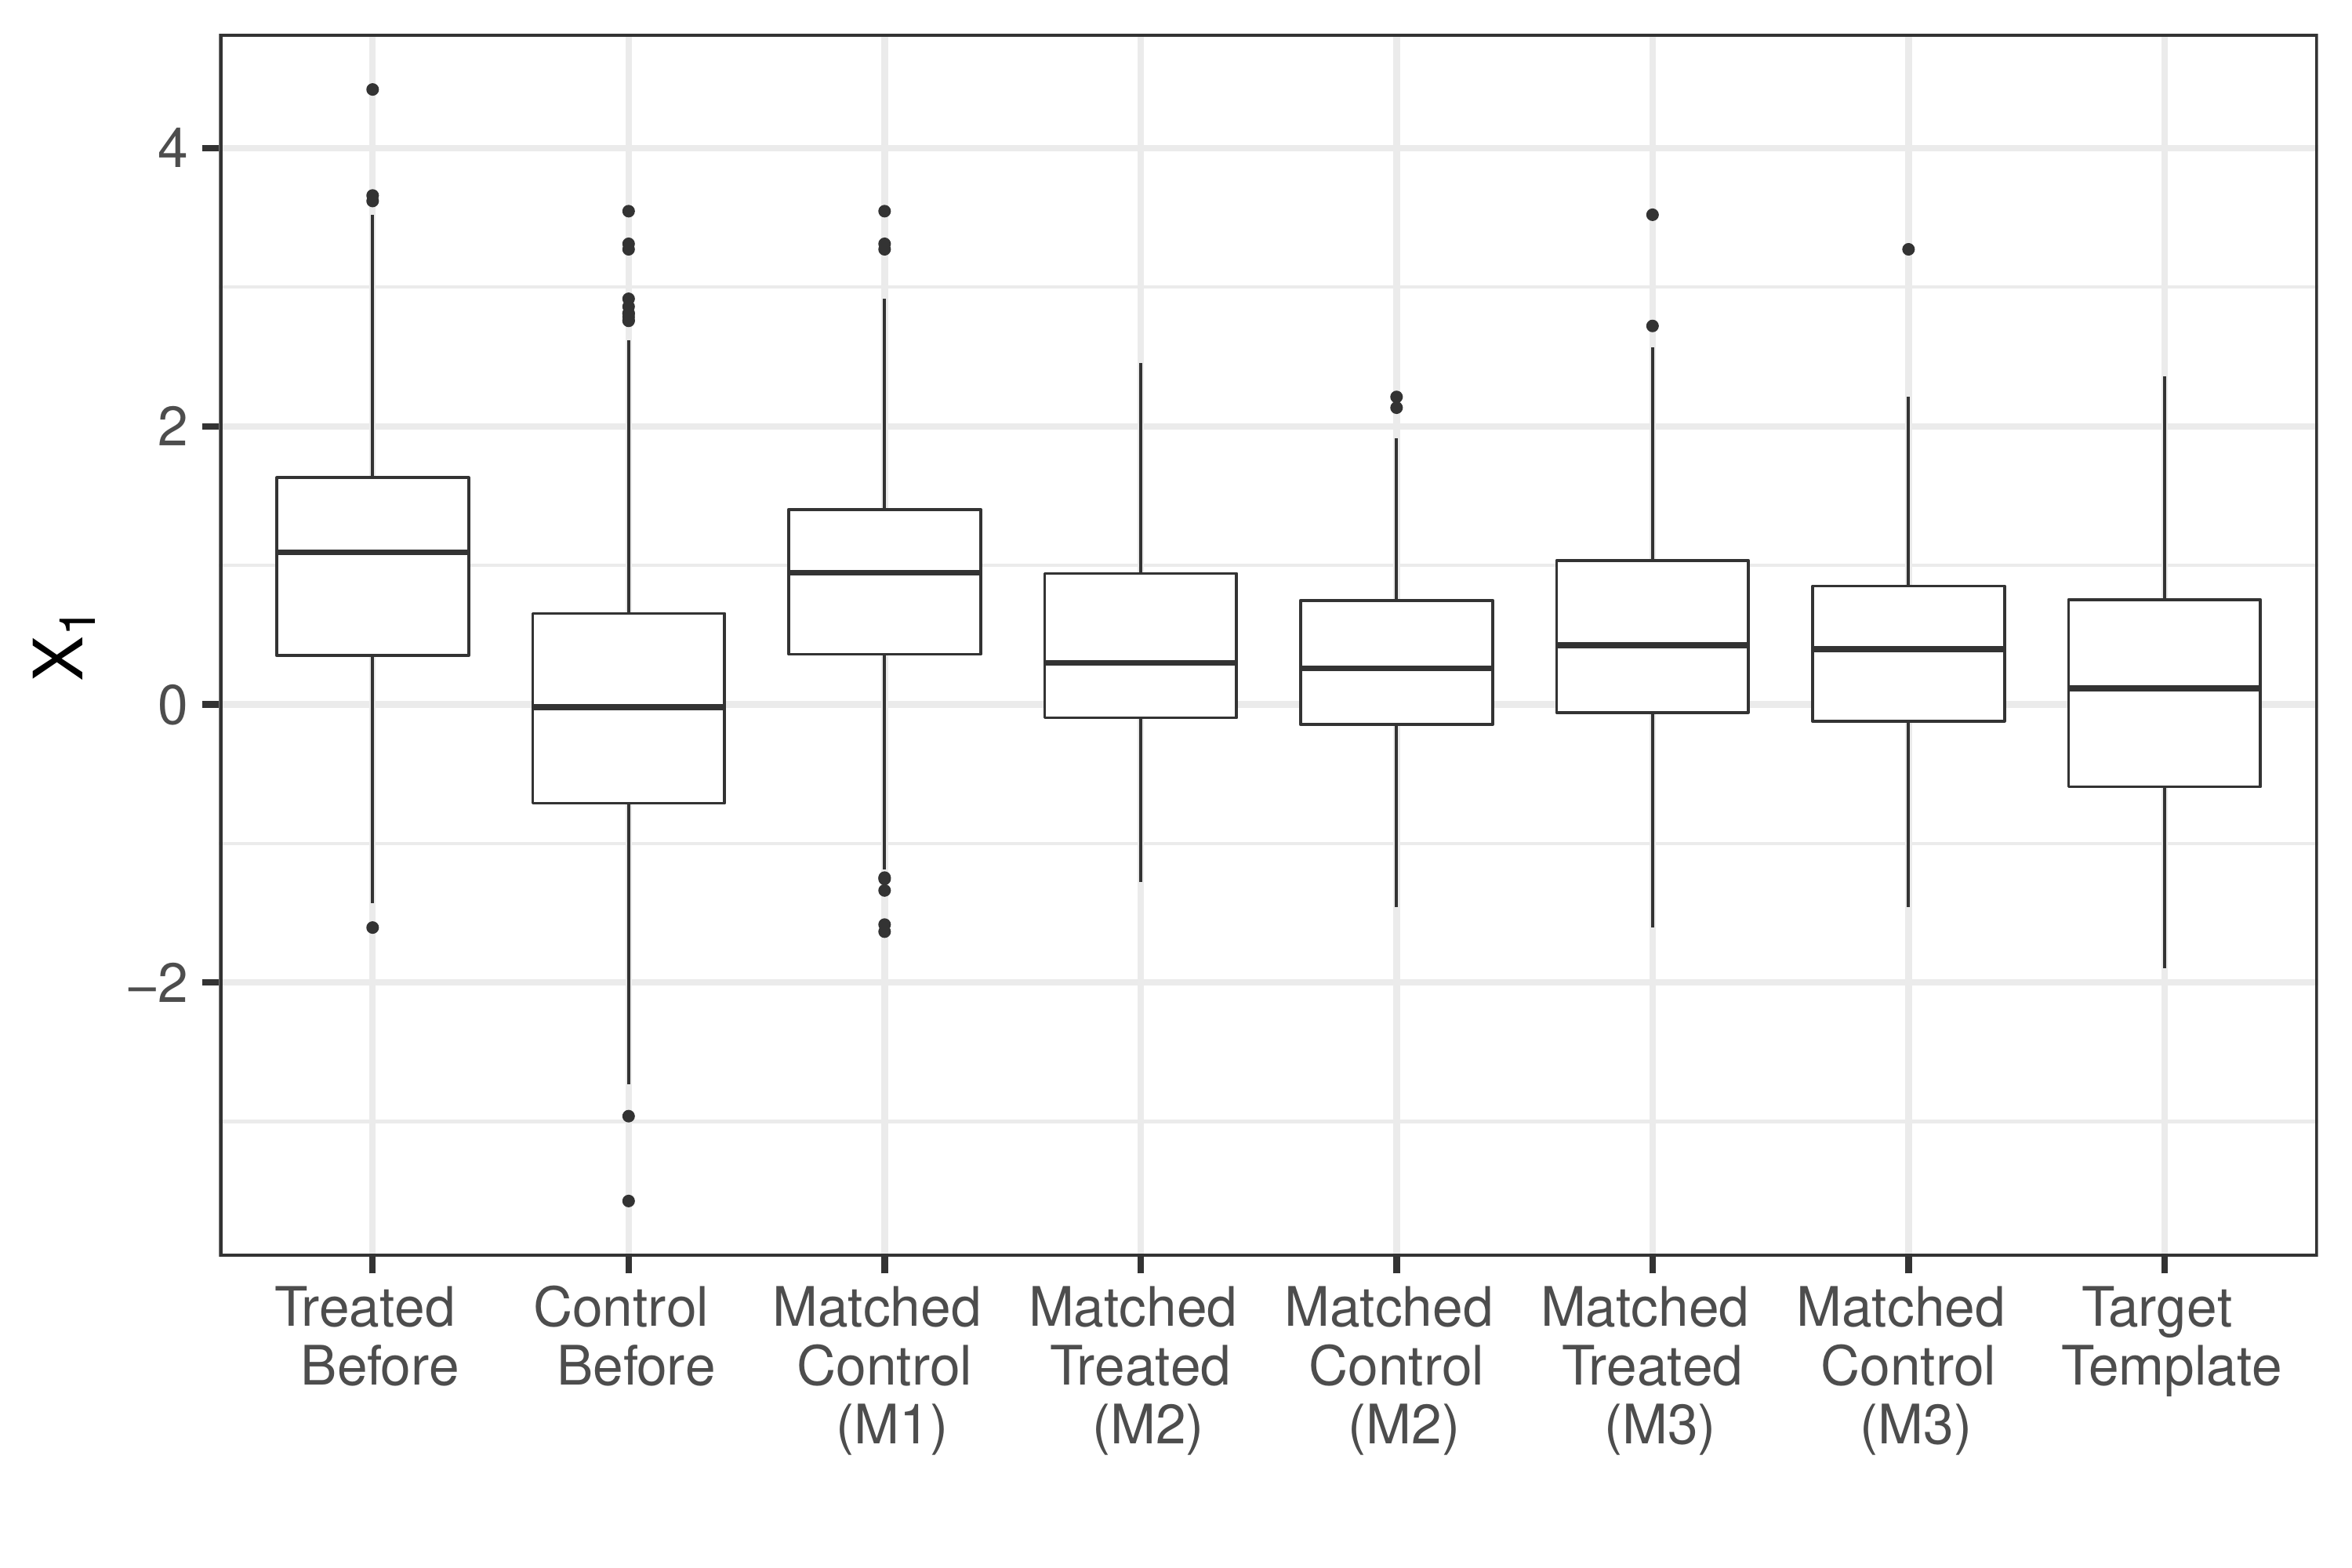}}
     \subfloat{\includegraphics[width = 0.49\columnwidth]{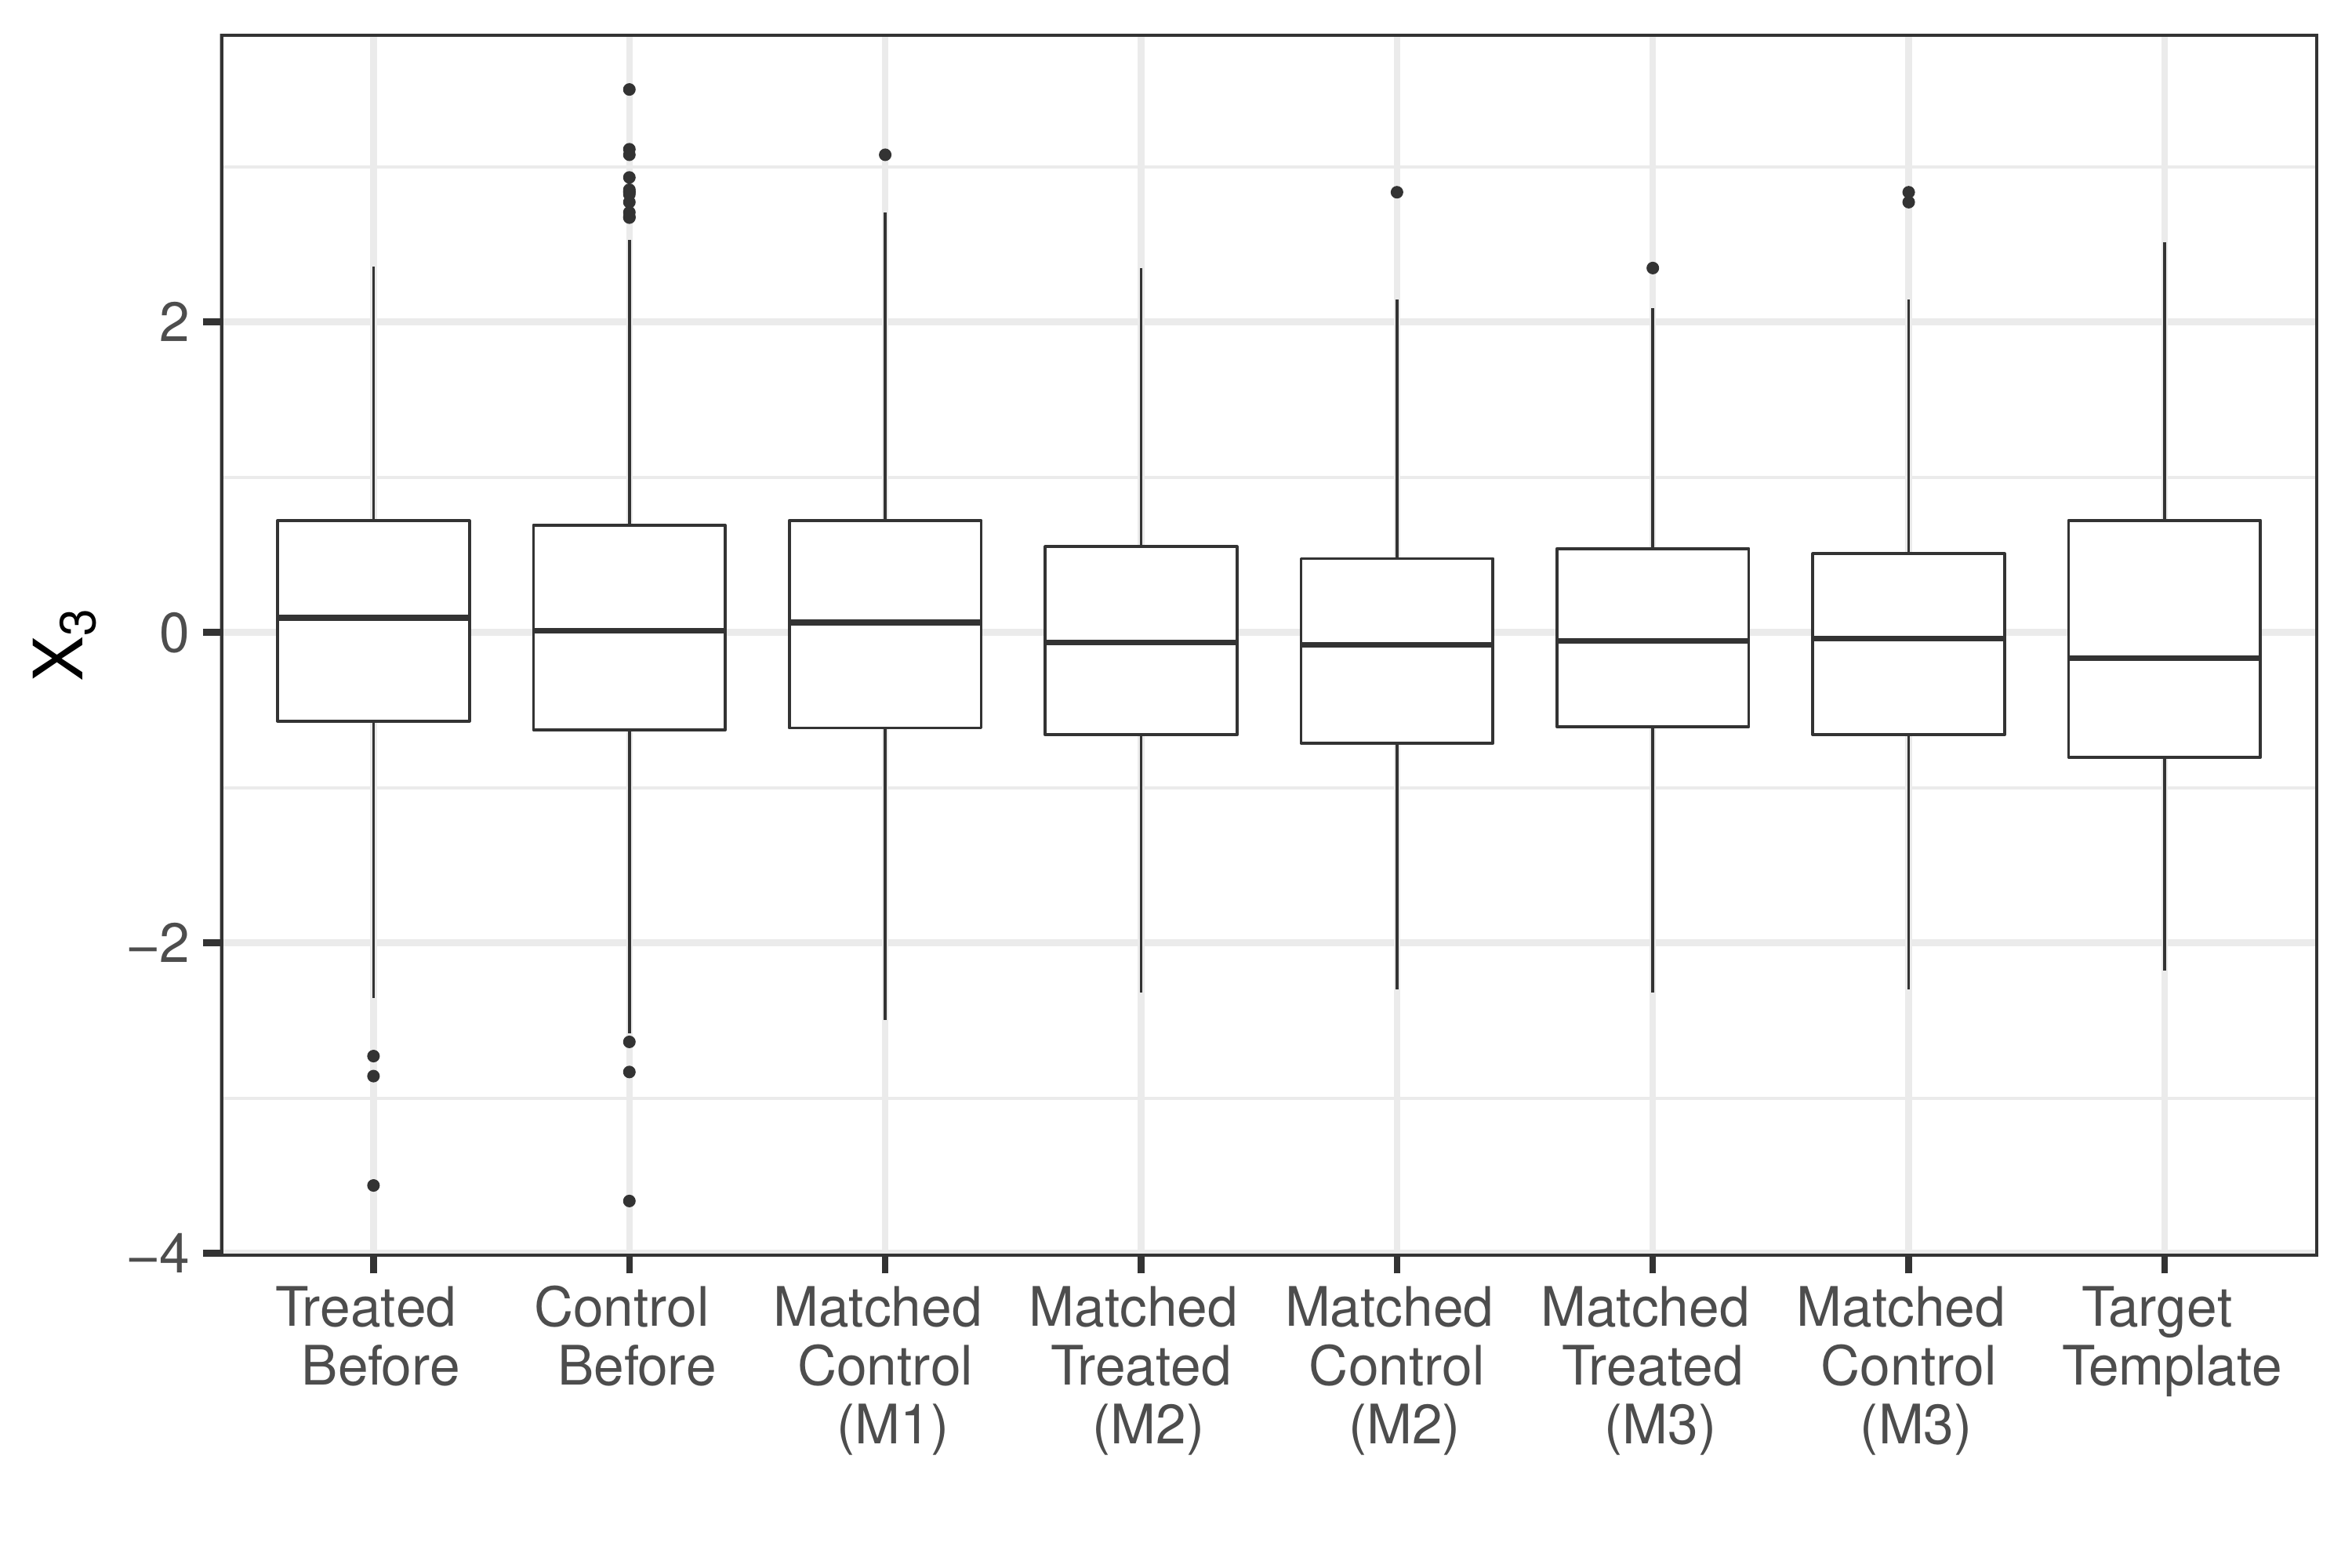}}
     \caption{Comparing the distributions of covariates $X_1$ (left panel) and $X_3$ (right panel) in three matched comparisons. Match $\textsf{M1}$ }
\label{fig: illustrative example}
\end{figure}
